# Supplementary material for: Variable Selection with Rigorous Uncertainty Quantification using Deep Bayesian Neural Networks: Posterior Concentration and Bernstein-von Mises Phenomenon
Source: arXiv:1912.01189 source file (2019-12-03)
Supplement: Supplementary file 1 [file supp.pdf]

# Supplementary Material for Variable Selection with Rigorous Uncertainty Quantification using Deep Bayesian Neural Networks

## Contents


**A Additional Background** **2**

A.1 Rectified Linear Unit (ReLU) Neural Network in Matrix Notation . . . . . . . . . . 2

A.2 ReLU Network in the reproducing kernel Hilbert space (RKHS) . . . . . . . . . . . 3

A.3 Bayesian Learning of Deep ReLU Neural Network . . . . . . . . . . . . . . . . . . 3

**B Proofs for Posterior Consistency** **4**

B.1 Proof for Theorem 1 . . . . . . . . . . . . . . . . . . . . . . . . . . . . . . . . . . 4

**C Proofs for Bernstein-von Mises (BvM) Phenomenon** **6**

C.1 Background: Semi-parametric BvM Theorem for Smooth Functionals . . . . . . . 6

C.2 Preliminary I: Notations and Basic Setup . . . . . . . . . . . . . . . . . . . . . . . 7

C.3 Preliminary II: Proof Strategy and Preliminary Theorems . . . . . . . . . . . . . . 8

C.4 Proof for Theorem 2 . . . . . . . . . . . . . . . . . . . . . . . . . . . . . . . . . . 9

C.5 Proof for Theorem 3 . . . . . . . . . . . . . . . . . . . . . . . . . . . . . . . . . . 11

**D Additional Proofs** **13**

D.1 Proof for Theorem C.2 . . . . . . . . . . . . . . . . . . . . . . . . . . . . . . . . . 13

D.2 Proof for Theorem C.3 . . . . . . . . . . . . . . . . . . . . . . . . . . . . . . . . . 17

**E Lemmas and Propositions** **19**

# A Additional Background

## A.1 ReLU Neural Network in Matrix Notation

Given a sample $\{y_i, \mathbf{x}_i\}_{i=1}^n$, the neural network predictions $\mathbf{f}_{n\times 1} = [f(\mathbf{x}_1), \dots, f(\mathbf{x}_n)]^\top$ can be represented as a $n \times 1$ vector in terms of its weight matrices. This matrix representation is mathematically convenient and provides important insight into how the data flow through the layers to interact with different components of the model. Interestingly, under the ReLU activation function, $\mathbf{f}_{n\times 1}$ can be written as a linear product of model weight matrices despite the fact that $f(\mathbf{x})$ itself is an nonlinear model. To keep the notation simple, in this section we will omit the bias term $b_0$. However we note that it can always be added back to the model by augmenting the feature matrix $\mathbf{\Phi}_{n\times K}$ (defined below) with a column vector of 1's.

We first consider the one-layer ReLU network $f(\mathbf{x}) = \beta^\top \sigma(\mathcal{W}_1 \mathbf{x})$. For a single hidden unit, the ReLU activation output is $\sigma(\mathcal{W}_{1,k}\mathbf{x}) = I(\mathcal{W}_{1,k}\mathbf{x} > 0) * \mathcal{W}_{1,k}\mathbf{x}$, and the ReLU output of the entire $K$-unit hidden layer is a $K \times 1$ vector $\sigma(\mathcal{W}_1\mathbf{x}) = S_{1,\mathbf{x}}\, \mathcal{W}_1\mathbf{x}$, where $S_{1,\mathbf{x}}$ is a $K \times K$ diagonal matrix with indicator functions $I(\mathcal{W}_{1,k}\mathbf{x} > 0)$ on the diagonal. As a result, the one-layer ReLU network evaluated at a single observation $\mathbf{x}_i$ is:

$$f(\mathbf{x}_i) = \beta^\top S_{1,\mathbf{x}_i} \mathcal{W}_1 \mathbf{x}_i.$$

To express $\mathbf{f}_{n\times 1} = [f(\mathbf{x}_1), \dots, f(\mathbf{x}_n)]^\top$, we define data matrix $\mathbf{X}$, weight matrix $\mathbf{W}_1$ and activation matrix $\mathbf{S}_1$ such that:

$$\mathbf{f}_{n\times 1} = \mathbf{\Phi}_{\mathcal{W}} \boldsymbol{\beta} = (\mathbf{X}\mathbf{W}_1\mathbf{S}_1)\boldsymbol{\beta}, \tag{1}$$

where we have defined $\mathbf{\Phi}_{\mathcal{W}, n\times K} = \mathbf{X}\mathbf{W}_1\mathbf{S}_1$ the matrix of hidden features, and

$$\mathbf{X} = \begin{bmatrix} \mathbf{x}_1 & 0 & \dots & 0 \\ 0 & \mathbf{x}_2 & \dots & 0 \\ \dots & & & \\ 0 & 0 & 0 & \mathbf{x}_n \end{bmatrix}_{n\times nP}, \quad \mathbf{W}_1 = \mathcal{W}_1 \otimes \mathbf{I}_n = \begin{bmatrix} \mathcal{W}_1 & 0 & \dots & 0 \\ 0 & \mathcal{W}_1 & \dots & 0 \\ \dots & & & \\ 0 & 0 & 0 & \mathcal{W}_1 \end{bmatrix}_{nP\times nK}, \quad \mathbf{S}_1 = \begin{bmatrix} S_{1,\mathbf{x}_1} \\ S_{1,\mathbf{x}_2} \\ \vdots \\ \dots \\ S_{1,\mathbf{x}_n} \end{bmatrix}_{nK\times K}.$$

To express $\mathbf{f}_{n\times 1}$ for a deep ReLU network $f(\mathbf{x}) = \beta^\top(\sigma\mathcal{W}_L \dots (\sigma\mathcal{W}_1\mathbf{x}))$, we notice a $L$-layer ReLU neural network evaluated at a single observation is expressed as:

$$f(\mathbf{x}) = \beta^\top \Big(\prod_{l=L}^{1} S_{l,\mathbf{x}} \mathcal{W}_l\Big)\, \mathbf{x}$$

using the short-hand notation $\prod_{l=L}^1 M_l = M_L M_{L-1} \dots M_2 M_1$. Here $S_{l,\mathbf{x}}$ is a $K \times K$ diagonal matrice with indicator functions $I(\mathcal{W}_{l,k}\sigma\mathcal{W}_{l-1}\dots\sigma\mathcal{W}_1\mathbf{x} > 0)$ on the diagonal. As a result:

$$\mathbf{f}_{n\times 1} = \mathbf{\Phi}_{\mathcal{W}}\beta = \Big(\mathbf{X}\big(\prod_{l=1}^{L} \mathbf{W}_l \mathbf{S}_l\big)\Big)\beta, \tag{2}$$

where $\mathbf{\Phi}_{\mathcal{W}, n\times K} = \mathbf{X}(\prod_{l=1}^L \mathbf{W}_l\mathbf{S}_l)$ is the matrix of hidden features at the output layer, and we have denoted $\mathbf{W}_l = \mathcal{W}_l \otimes \mathbf{I}_n$ and $\{\mathbf{S}_l\}_{l=1}^{L-1}$, $\mathbf{S}_L$ as:

$$\mathbf{S}_l = \begin{bmatrix} S_{l,\mathbf{x}_1} & 0 & \dots & 0 \\ 0 & S_{l,\mathbf{x}_2} & \dots & 0 \\ \dots & & & \\ 0 & 0 & 0 & S_{l,\mathbf{x}_n} \end{bmatrix}_{nK\times nK}, \quad \mathbf{S}_L = \begin{bmatrix} S_{L,\mathbf{x}_1} \\ S_{L,\mathbf{x}_2} \\ \vdots \\ \dots \\ S_{L,\mathbf{x}_n} \end{bmatrix}_{nK\times K}.$$

It is worth noting that the gradient function of a ReLU network $\partial_p \mathbf{f}_{n\times 1} = [\frac{\partial}{\partial x_p} f(\mathbf{x}_1), \dots, \frac{\partial}{\partial x_p} f(\mathbf{x}_n)]^\top$ can also be expressed as a linear product of matrices. Specificially, since ReLU network is expressed as $\mathbf{f} = \mathbf{\Phi}\beta$ with $\mathbf{\Phi} = \mathbf{X}(\prod_{l=1}^L \mathbf{W}_l\mathbf{S}_l)\beta$, its derivative can be written as:

$$\partial_p \mathbf{f}_{n\times 1} = (\partial_p \Phi)\beta = \Big(\mathbf{W}_{1,p}\mathbf{S}_1\big(\prod_{l=2}^{L} \mathbf{W}_l\mathbf{S}_l\big)\Big)\beta$$

where $\mathbf{W}_{1,p}$ is a $n \times nK$ matrix such that $\mathbf{W}_{1,p} = \mathbf{I}_n \otimes \mathcal{W}_{1,p}$. Correspondingly, the empirical norm of the gradient function can be written as:

$$\psi_p(f) = ||\frac{\partial}{\partial x_p} f||_n^2 = \frac{1}{n}||\partial_p \mathbf{f}_{n\times 1}||_2^2 = \frac{1}{n}\beta^\top(\partial_p\Phi)^\top(\partial_p\Phi)\beta,$$

which is of a quadratic form with respect to a $K \times K$ "gradient kernel matrix" $(\partial_p\Phi)^\top(\partial_p\Phi)$.

### A.2 ReLU Network in the RKHS

It is important to notice that the function space $\mathcal{F}(L, K, S, B)$ corresponds to a reproducing kernel Hilbert space (RKHS) [3, 2]. Specifically, notice that if we focus on the output layer, then every $f \in \mathcal{F}(L, K, S, B)$ can be written as

$$f(\mathbf{x}) = \phi_{\mathcal{W}}(\mathbf{x})^\top\beta = \sum_{k=1}^{K}\beta_k\phi_k(\mathbf{x}|\mathcal{W}),$$

where $\phi_k(\mathbf{x}|\mathcal{W}) = \mathcal{W}_{k,L}\Big[\circ_{l=1}^{L-1}(\sigma\mathcal{W}_l)\circ\mathbf{x}\Big]$ are the $K$ "basis functions" at the output layer that are formed by the hidden neurons.

Consequently, $\mathcal{F}(L, K, S, B)$ corresponds to a RKHS $\mathcal{H}$ equipped with positive definite kernel $k_{\mathcal{W}}(\mathbf{x}, \mathbf{x}') = \phi_{\mathcal{W}}(\mathbf{x})^\top\phi_{\mathcal{W}}(\mathbf{x}') = \sum_{k=1}^{K}\phi_k(\mathbf{x}|\mathcal{W})\phi_k(\mathbf{x}'|\mathcal{W})$, and the hidden weights $\mathcal{W}$ can be regarded as the hyper-parameters for this RKHS kernel [3]. For two functions in this RKHS $f(\mathbf{x}) = \phi_{\mathcal{W}}(\mathbf{x})^\top\beta_f$ and $g(\mathbf{x}) = \phi_{\mathcal{W}}(\mathbf{x})^\top\beta_g$, the inner product in $\mathcal{H}$ is defined as:

$$\langle f, g\rangle_{\mathcal{H}} = \beta_f^\top\beta_g,$$

i.e., we can interpret the output-layer weights $\beta$ as a "representer" of $f$ in $\mathcal{H}$. It is important to verify that the above definition of $\langle ., .\rangle_{\mathcal{H}}$ indeed gives rise to the reproducing property:

$$\langle f, k(\mathbf{x}, .)\rangle_{\mathcal{H}} = \beta_f^\top\phi_{\mathcal{W}}(\mathbf{x}) = f(\mathbf{x}),$$

which can be seen easily by noticing that $k_{\mathcal{W}}(\mathbf{x}, .) = \phi_{\mathcal{W}}(\mathbf{x})^\top\phi_{\mathcal{W}}(.)$ is an element in $\mathcal{H}$ with its "$\beta$" being $\phi_{\mathcal{W}}(\mathbf{x})$. Finally, the quadratic norm in this space is defined by $||f||_{\mathcal{H}}^2 = \sum_{k=1}^{K}\beta_{f,w}^2 = ||\beta_f||_2^2$ [2].

To compute the kernel function $k_{\mathcal{W}}$ and the corresponding kernel matrix $\mathbf{K}_{\mathcal{W}}$ for a ReLU network, we recall that, for the single-layer ReLU network $f(\mathbf{x}) = \beta\sigma(\mathcal{W}_1\mathbf{x})$, the corresponding basis function is a $K \times 1$ vector $\phi_{\mathcal{W}}(\mathbf{x})_{K\times 1} = \sigma(\mathcal{W}_1\mathbf{x}) = S_{1,\mathbf{x}}\mathcal{W}_1\mathbf{x}$. so we can write $k_{\mathcal{W}}$ in terms of $\phi_{\mathcal{W}}$ as:

$$k_{\mathcal{W}}(\mathbf{x}, \mathbf{x}') = \phi_{\mathcal{W}}(\mathbf{x})^\top\phi_{\mathcal{W}}(\mathbf{x}') = \mathbf{x}^\top\mathcal{W}_1^\top S_{1,\mathbf{x}}\ S_{1,\mathbf{x}'}\mathcal{W}_1\mathbf{x}'.$$

Similarly, $k_{\mathcal{W}}$ for a $L$-layer ReLU network is:

$$k_{\mathcal{W}}(\mathbf{x}, \mathbf{x}') = \phi_{\mathcal{W}}(\mathbf{x})^\top\phi_{\mathcal{W}}(\mathbf{x}') = \mathbf{x}^\top(\prod_{l=L}^{1}S_{l,\mathbf{x}}\mathcal{W}_l)^\top(\prod_{l=L}^{1}S_{l,\mathbf{x}'}\mathcal{W}_l)\mathbf{x}'.$$

To express the kernel matrix $\mathbf{K}_{\mathcal{W},n\times n}$, recall the matrix of basis functions $\mathbf{\Phi}_{\mathcal{W},n\times K} = [\phi_{\mathcal{W}}(\mathbf{x}_1), \dots, \phi_{\mathcal{W}}(\mathbf{x}_n)]^\top$ can be expressed compactly as $\mathbf{\Phi}_{\mathcal{W}} = \mathbf{X}\mathbf{W}_1\mathbf{S}_1$ for a single-layer network, and $\mathbf{\Phi}_{n\times K} = \mathbf{X}(\prod_{l=1}^{L}\mathbf{W}_l\mathbf{S}_l)$ for a deep ReLU network. So the kernel matrices $\mathbf{K}_{\mathcal{W}}$ for a single-layer and a deep ReLU network are, respectively:

$$\mathbf{K}_{\mathcal{W}} = \mathbf{\Phi}\mathbf{\Phi}^\top = \mathbf{X}\mathbf{W}_1\mathbf{S}_1\mathbf{S}_1^\top\mathbf{W}_1^\top\mathbf{X}^\top, \quad \mathbf{K}_{\mathcal{W}} = \mathbf{\Phi}\mathbf{\Phi}^\top = \mathbf{X}(\prod_{l=1}^{L}\mathbf{W}_l\mathbf{S}_l)(\prod_{l=1}^{L}\mathbf{W}_l\mathbf{S}_l)^\top\mathbf{X}^\top.$$

### A.3 Bayesian Learning of Deep ReLU Neural Network

It is well-known that for some common choices of $\Pi(\beta)$, $\Pi(f)$ corresponds to a (conditional) Gaussian process (GP) [14]. Specifically, by placing independent and identically distributed (i.i.d.) Gaussian prior $N(0, \frac{1}{K})$ on $\beta$ and $N(0, \sigma_{b_0}^2)$ on $b_0$, the neural network model $f(.) = \phi_{\mathcal{W}}(.)^\top\beta$ is equal

in distribution to Gaussian process with kernel function $k_{\mathcal{W}}(\mathbf{x}, \mathbf{x}') = \frac{1}{K}\phi_{\mathcal{W}}(\mathbf{x})^\top \phi_{\mathcal{W}}(\mathbf{x}') + \sigma^2_{b_0}$, i.e., $\Pi(f|\mathcal{W}) = GP(f|0, k_{\mathcal{W}})$.

As a result, under the conditional Gaussian process (GP) representation, the prior distribution for $f$ can be written as:

$$\Pi(f, \mathcal{W}) = \Pi(f|\mathcal{W})\Pi(\mathcal{W}) = GP(f|0, k_{\mathcal{W}})\Pi(\mathcal{W}), \tag{3}$$

The conditional GP representation in (3) is important for analyzing the asymptotic behavior of the Bayesian neural network. It suggests that, if the behavior of the conditional posterior $\Pi_n(f|\mathcal{W})$ does not change drastically under $\Pi_n(\mathcal{W})$, then the asymptotic behavior of $\Pi_n(f, \mathcal{W})$ is analogous to that of a Gaussian process, whose theoretical properties are well-understood in the literature [22, 6]. In Section D.1 - D.2, we take advantage of this representation to show an BvM phenomenon (i.e. asymptotic normality) for the posterior distribution of variable importance for a wide range of choices for $\Pi(\mathcal{W})$.

# B Proofs for Posterior Consistency

## B.1 Proof for Theorem 1

*Proof.* Denote $A_n = \{f : ||f - f_0||^2_n > M_n\epsilon_n\}$ and $B_n = \{f : |\psi_p(f) - \Psi_p(f_0)| > M_n\epsilon_n\}$, then showing the statement in Theorem 1 is equivalent to showing $\Pi_n(B_n) \to 0$.

Specifically, we assume below three facts hold:

**Fact 1** $|\psi_p(f) - \psi_p(f_0)| \leq ||\frac{\partial}{\partial x_p} f - \frac{\partial}{\partial x_p} f_0||^2_n$

**Fact 2** $\sup_{p\in\{1,\dots,P\}} ||\frac{\partial}{\partial x_p} f - \frac{\partial}{\partial x_p} f_0||^2_n \leq C * ||f - f_0||^2_n$ for some constant $C$.

**Fact 3** $\sup_{p\in\{1,\dots,P\}} |\psi_p(f_0) - \Psi_p(f_0)| \lesssim ||f - f_0||^2_n$.

Because if above facts hold, we then have

$$\begin{aligned}
\sup_{p\in\{1,\dots,P\}} |\psi_p(f) - \Psi_p(f_0)| &\leq \sup_{p\in\{1,\dots,P\}} |\psi_p(f) - \psi_p(f_0)| + \sup_{p\in\{1,\dots,P\}} |\psi_p(f_0) - \Psi_p(f_0)| \\
&\leq \sup_{p\in\{1,\dots,P\}} ||\frac{\partial}{\partial x_p} f - \frac{\partial}{\partial x_p} f_0||^2_n + \sup_{p\in\{1,\dots,P\}} |\psi_p(f_0) - \Psi_p(f_0)| \\
&\leq C * ||f - f_0||^2_n + \sup_{p\in\{1,\dots,P\}} |\psi_p(f_0) - \Psi_p(f_0)| \\
&\lesssim ||f - f_0||^2_n,
\end{aligned}$$

it then follows that:

$$E_0\Pi_n\Big(\sup_{p\in\{1,\dots,P\}} |\psi_p(f) - \Psi_p(f_0)| \geq M_n\epsilon_n\Big) \lesssim E_0\Pi_n\Big(||f - f_0||^2_n \geq M'_n\epsilon_n\Big) \to 0.$$

We now show Facts 1-3 are true:

- **Fact 1** follows simply from the triangular inequality:

$$\begin{aligned}
|\psi_p(f) - \psi_p(f_0)| &= \Big| ||\frac{\partial}{\partial x_p} f||^2_n - ||\frac{\partial}{\partial x_p} f_0||^2_n \Big| \\
&= \max\Big\{ ||\frac{\partial}{\partial x_p} f||^2_n - ||\frac{\partial}{\partial x_p} f_0||^2_n,\ ||\frac{\partial}{\partial x_p} f_0||^2_n - ||\frac{\partial}{\partial x_p} f||^2_n \Big\} \leq ||\frac{\partial}{\partial x_p} f_0 - \frac{\partial}{\partial x_p} f||^2_n.
\end{aligned}$$

- **Fact 2**. First establish some notation. Given data $\{\mathbf{x}_i, y_i\}_{i=1}^n$, denote $\mathbf{f}$ and $\mathbf{f}_0$ the $n \times 1$ vectors with their elements being $f(\mathbf{x}_i)$, $f_0(\mathbf{x}_i)$, respectively. We then have $||f - f_0||^2_n = ||\mathbf{f} - \mathbf{f}_0||^2_2$. Furthermore, since $f, f_0 \in \mathcal{F}(L, W, S, B)$, there exisits sets of weight matrices $\{\mathbf{W}_l, \mathbf{S}_l\}_{l=1}^L$, $\{\mathbf{W}_{0,l}, \mathbf{S}_{0,l}\}_{l=1}^L$ and output weights $\boldsymbol{\beta}, \boldsymbol{\beta}_0$ such that $\mathbf{f} = \mathbf{X}\mathbf{W}_1\mathbf{S}_1(\prod_{l=2}^L \mathbf{W}_l\mathbf{S}_l)\boldsymbol{\beta}$ and $\mathbf{f}_0 =$

$\mathbf{X}\mathbf{W}_{0,1}\mathbf{S}_{0,1}(\prod_{l=2}^{L}\mathbf{W}_{0,l}\mathbf{S}_{0,l})\boldsymbol{\beta}_0$. To keep the notation simple, we write for $\mathbf{f}$ its the input weights as $\mathbf{W}$, and the product of weight matrices after the input layer as $\mathbf{D} = \mathbf{S}_1(\prod_{l=2}^{L}\mathbf{W}_l\mathbf{S}_l)\boldsymbol{\beta}$, such that $\mathbf{f}$ and $\mathbf{f}_0$ can be written as:

$$\mathbf{f} = \mathbf{X}\mathbf{W}\mathbf{D}, \quad \mathbf{f}_0 = \mathbf{X}\mathbf{W}_0\mathbf{D}_0$$

where recall $\mathbf{X}$ is a $n \times nP$ block diagonal matrix with $1 \times p$ vectors $\mathbf{x}_i$'s on the diagonal. Furthermore, by the definition of gradient functions for ReLU network, we can write the $n \times 1$ vectors of gradient functions as:

$$\partial_p\mathbf{f} = \mathbf{W}_p\mathbf{D}, \quad \partial_p\mathbf{f}_0 = \mathbf{W}_{0,p}\mathbf{D}_0,$$

where $\mathbf{W}_p = \mathbf{I}_n \otimes \mathbf{w}_p, \mathbf{W}_{0,p} = \mathbf{I}_n \otimes \mathbf{w}_{0,p}$ are $n \times nK$ block diagonal matrices. Notice that $||\frac{\partial}{\partial x_p}f - \frac{\partial}{\partial x_p}f_0||_n^2 = ||\partial_p\mathbf{f} - \partial_p\mathbf{f}_0||_2^2$. Finally, we will denote $\mathbb{X} = [\mathbf{X}^\top, \dots, \mathbf{X}^\top]^\top$ a $nP \times nP$ matrix that is formed by stacking $\mathbf{X}$ for $P$ times.

Consequently:

$$\begin{aligned}
\sup_{p\in\{1,\dots,P\}} ||\frac{\partial}{\partial x_p}f - \frac{\partial}{\partial x_p}f_0||_n^2 &\leq \sum_{p=1}^{P} ||\frac{\partial}{\partial x_p}f - \frac{\partial}{\partial x_p}f_0||_n^2 \\
&= \sum_{p=1}^{P} ||\mathbf{W}_p\mathbf{D} - \mathbf{W}_{0,p}\mathbf{D}_0||_2^2 = ||\mathbf{W}\mathbf{D} - \mathbf{W}_0\mathbf{D}_0||_2^2 \\
&\leq ||\mathbb{X}^{-1}\mathbb{X}(\mathbf{W}\mathbf{D} - \mathbf{W}_0\mathbf{D}_0)||_2^2 \leq ||\mathbb{X}^{-1}||_2^2||\mathbb{X}\mathbf{W}\mathbf{D} - \mathbb{X}\mathbf{W}_0\mathbf{D}_0||_2^2 \\
&= P * ||\mathbb{X}^{-1}||_2^2||\mathbf{X}\mathbf{W}\mathbf{D} - \mathbf{X}\mathbf{W}_0\mathbf{D}_0||_2^2 = P * ||\mathbb{X}^{-1}||_2^2||f - f_0||_n^2 \\
&\leq \frac{P}{c_x}||f - f_0||_n^2.
\end{aligned}$$

The equality on the fourth line follows since $||\mathbb{X}(\mathbf{W}\mathbf{D} - \mathbf{W}_0\mathbf{D}_0)||_2^2 = P * ||\mathbf{X}(\mathbf{W}\mathbf{D} - \mathbf{W}_0\mathbf{D}_0)||_2^2$, due to the fact that $\mathbb{X}$ is formed by stacking the $\mathbf{X}$ matrix $P$ times. We can assume without loss of generality that for $\mathbf{x}_i = \{x_{i,p}\}_{p=1}^P$, $x_{i,p}$ is always bounded away from zero by a small constant $c_x > 0$, such that $x_{i,p} \geq c_x \forall i, p$. Then the inequality on the last line follows since $||\mathbb{X}^{-1}||_2$ is bounded by $\frac{1}{c_x}$. This is because $||\mathbb{X}^{-1}||_2 = \lambda_{max}(\mathbb{X}^{-1}) = 1/\lambda_{min}(\mathbb{X})$, and $\mathbb{X}$ can be reordered (through column permutation) into a block matrix with $P \times P$ diagonal matrices $\mathbf{X}_i = diag(x_{i,1}, \dots, x_{i,p})$, such that: $\mathbb{X} = \begin{bmatrix} \mathbf{X}_1 & \mathbf{X}_2 & \dots & \mathbf{X}_n \\ \mathbf{X}_1 & \mathbf{X}_2 & \dots & \mathbf{X}_n \\ \dots & \dots & \dots & \dots \\ \mathbf{X}_1 & \mathbf{X}_2 & \dots & \mathbf{X}_n \end{bmatrix}$. Since eigenvalues of $\mathbb{X}$ is invariant under column permutation, and eigenvalue of a block matrix is the eigenvalues of the matrix blocks on the diagonal, we see that $\lambda_{min}(\mathbb{X}) = min_{i,p}(x_{i,p}) \geq c_x$. Consequently, since $\frac{P}{c_x} = O_p(1)$, we have shown that for some constant $C$:

$$\sup_{p\in\{1,\dots,P\}} ||\frac{\partial}{\partial x_p}f - \frac{\partial}{\partial x_p}f_0||_n^2 \leq C * ||f - f_0||_n^2$$

- **Fact 3** follows from standard Bernstein-type concentration inequality (see, e.g. Lemma 18 of [18]). Specifically, for $|\frac{\partial}{\partial x_p}f_0(\mathbf{x})|^2$ a random variable with respect to probability measure $P(\mathbf{x})$ that is bounded by $L$. Given $n$ i.i.d. samples $\{|\frac{\partial}{\partial x_p}f_0(x_i)|^2\}_{i=1}^n$, recall that $\hat{\psi}(f_0) = \frac{1}{n}\sum_{i=1}^n |\frac{\partial}{\partial x_p}f_0(x_i)|^2$ and $\psi(f_0) = E(\frac{\partial}{\partial x_p}f_0)$, then with probability $1 - \eta$:

$$|\hat{\psi}(f_0) - \psi(f_0)| \leq n^{-\frac{1}{2}} * \big(2\sqrt{2} * L * log(2/\eta)\big),$$

that is, $|\hat{\psi}(f_0) - \psi(f_0)| \to 0$ at rate of $O(n^{-\frac{1}{2}})$. Notice that $O(n^{-\frac{1}{2}})$ is the optimal parametric rate that cannot be surpassed by the convergence speed of the ReLU networks (recall the typical convergence rate is $\epsilon_n \asymp n^{-\frac{\beta}{2\beta+\delta}} * log(n)^\gamma$ for some $\delta > 0$ and $\gamma > 1$). Therefore we have:

$$\sup_{p\in\{1,\dots,P\}} |\psi_p(f_0) - \Psi_p(f_0)| \lesssim ||f - f_0||_n^2.$$

□

## C Proofs for BvM Phenomenon

### C.1 Background: Semi-parametric BvM Theorem for Smooth Functionals

In this section, we provide background on a general semi-parametric BvM theorem for smooth nonlinear functionals [7]. In nonparametric regression, the regression function $f \in \mathcal{F}$ is infinite-dimensional and the asymptotic distribution of $f$ in this case is in general difficult to characterize [8]. However, in practical applications, we are mostly interested in a finite-dimensional parameter $\psi : \mathcal{F} \rightarrow \mathbb{R}^d$ whose asymptotic distribution is easier to reason with. For example, a cumulative distribution function at a fixed point $F(x_0) = \int \mathbb{I}(x < x_0) f(x) dx$ [16].

To this end, a series of work by [4, 16, 7] provided general sufficient conditions for BvM theorem in smooth functionals under general models. These results show that, if the functional of interest $\psi$ and the model log likelihood $l_n$ both satisfy certain smoothness conditions, then the marginal posterior of $\psi(f)$ concentrates at the rate $O(n^{-1/2})$, and furthermore, the marginal posterior distribution of $\sqrt{n}(\psi(f) - \hat{\psi})$ converges weakly to a $N(0, V_0)$ under the data-generation distribution $P_0$, where $\hat{\psi}$ is an efficient estimator of $\psi(f_0)$. Such properties have the implication that it allow the construction of credible regions for which have correct asymptotic frequentist coverage [6].

The main conditions are as below:

1. Locally Asymptotic Normal (LAN) Expansion of Likelihood Function $l_n(f)$:
$$l_n(f) - l_n(f_0) = -\frac{n}{2}||f - f_0||_n^2 + \sqrt{n} W_n(f - f_0). \tag{4}$$
2. Smoothness Expansion of Functional $\psi(f)$:
$$\psi(f) - \psi(f_0) = \langle \psi_1, f - f_0 \rangle_n + \frac{1}{2}\langle \psi_2(f - f_0), f - f_0 \rangle_n + o_p(\sqrt{n}). \tag{5}$$
3. Relation between $l_n(f)$ and $\psi(f)$:
For a posterior distribution $\Pi_n(f) = \Pi(f|\{y_i, \mathbf{x}_i\}_{i=1}^n)$ that concentrates around $f_0$ at rate $\epsilon_n$, i.e. $\Pi_n(f : ||f - f_0||_n \leq \epsilon_n) = 1 + o_p(1)$, define $A_n$ as the sequence of sets that receive majority of probability mass from $\Pi_n$, i.e.
$$\Pi_n(A_n) = \Pi_n(f \in A_n : ||f - f_0||_n \leq \epsilon_n) = 1 + o_p(1).$$
Assume there exists $w_n \in \mathcal{F}$ such that $W_n$ adopts a decomposition
$$W_n(f) = \langle w_n, f \rangle_n + \Delta_n(f),$$
where $w_n$ is the "representor" of $W_n$ such that $\langle w_n, f \rangle_n$ retains majority of information from $W_n(f)$, and $\Delta_n(f)$ is the corresponding residual term. It is required that both of these terms are sufficiently regular in the sense that they satisfy below two conditions:
$$\langle w_n, \psi_2(\psi_1) \rangle_n + \epsilon_n ||w_n||_n = o_p(\sqrt{n}), \tag{6}$$
$$\sup_{f \in A_n} |\Delta_n(\psi_2(f - f_0))| = o_p(1). \tag{7}$$

Then under some mild additional conditions, BvM is valid in below sense:

**Theorem C.1** (Semiparametric BvM Theorem)**.** *Let $W_n$, $w_n$ and $\psi$, $\psi_1$, $\psi_2$ as defined above. Furthermore, denote*
$$f_t = f - \frac{t}{\sqrt{n}}\Big(\psi_1 + \frac{1}{2}\psi_2(f - f_0)\Big) - \frac{t}{2n}\psi_2(w_n)$$
*and*
$$\hat{\psi} = \psi(f_0) + \frac{W_n(\psi_1)}{\sqrt{n}} + \frac{1}{2}\frac{\langle w_n, \psi_2(w_n) \rangle_n}{n}, \quad V_{0,n} = \Big|\Big|\psi_1 - \frac{1}{2}\frac{\psi_2(w_n)}{\sqrt{n}}\Big|\Big|_n^2$$

*Then the "moment generating function (MGF)" of $\sqrt{n}(\psi(f) - \hat{\psi})$ under posterior distribution $\Pi_n$ evaluated at the set $A_n$ such that $\Pi_n(A_n) = 1$ can be written as:*
$$E_n(e^{t\sqrt{n}(\psi(f) - \hat{\psi})}|A_n) = e^{o_p(1) + t^2 V_{0,n}/2} * \mathcal{I}_n, \quad where \quad \mathcal{I}_n = \frac{\int_{A_n} e^{l_n(f_t) - l_n(f_0)} d\Pi(f|\mathcal{W})}{\int_{A_n} e^{l_n(f) - l_n(f_0)} d\Pi(f|\mathcal{W})}$$

*Moreover, if* $V_{0,n} = ||\psi_1||_n^2 + o_p(1)$ *and* $\mathcal{I}_n = o_p(1)$*, then the posterior distribution* $\sqrt{n}(\psi(f) - \hat{\psi}_p)$ *is asymptotically normal with mean zero and variance* $||\psi_1||_n^2$*, i.e.*

$$\Pi_n\Big(\sqrt{n}(\psi(f) - \hat{\psi}_p)\Big) \rightsquigarrow N(0, ||\psi_1||_n^2) \tag{8}$$

*Proof.* [7], Theorem 2.1. □

Although the original theorem is stated under the scalar case, the generalization to multivariate case is straightforward, i.e., one only need to generalize $V_0$ to the corresponding matrix form following the definitition of $\psi_1$ [7].

### C.2 Preliminary I: Notations and Basic Setup

In this section, we set up the basic notations for showing semi-parametric BvM theorems for $\psi_p(f)$ in a nonparametric regression model. We will first verify the model likelihood $l_n(f) = -\frac{1}{2}\sum_{i=1}^n (y_i - f(\mathbf{x}_i))^2$ and the functional $\psi(f) = \langle H_p(f), f\rangle_n$ satisfy the three conditions for Theorem C.1, and by doing so, identify the expression for the technical terms $W_n$, $w_n$, $\psi_1$, $\psi_2$ that are relevant for deriving the asymptotic distribution of $\sqrt{n}(\psi(f) - \hat{\psi})$.

First verify (4) the LAN condition for model likelihood $l_n(f)$ and derive expression for $W_n$. Under independent Gaussian assumption, the likelihood for nonparametric regression adopts the LAN expansion:

$$l_n(f) - l_n(f_0) = -\frac{n}{2}||f - f_0||_n^2 + \sqrt{n}W_n(f - f_0)$$

where $||f - f_0||_n^2 = \frac{1}{n}\sum_{i=1}^n (f(\mathbf{x}_i) - f_0(\mathbf{x}_i))^2$, and $W_n$ is:

$$W_n(f) = \langle \sqrt{n}\epsilon, f\rangle_n = \frac{1}{n}\sum_{i=1}^n \sqrt{n}\epsilon_i * f(\mathbf{x}_i) \tag{9}$$

Now verify the rest of the two conditions, we consider two cases: the univariate case where $\psi_p(f) = ||\frac{\partial}{\partial x_p} f||_n^2$, to be used by the univariate BvM Theorem 2, and the multivariate case $\psi(f)_{P\times 1} = [||\frac{\partial}{\partial x_1} f||_n^2, \dots, ||\frac{\partial}{\partial x_P} f||_n^2]^\top$, to be used by the multivariate BvM Theorem 3..

#### Univariate Case

Now verify (5) the smoothness condition for functional of interest $\psi^c(f)$ and derive expressions for $\psi_1$, $\psi_2$. The centered quadratic norm of gradient $\psi_p^c(f) = \langle H_p(f), f\rangle_n - E(\langle H_p\,\omega, \omega\rangle_n)$ adopts the smoothness expansion:

$$\psi_p^c(f) - \psi_p^c(f_0) = \langle \psi_1, f - f_0\rangle_n + \frac{1}{2}\langle \psi_2(f - f_0), f - f_0\rangle_n + o_p(\sqrt{n}),$$

in which $\psi_1$, $\psi_2$ take the form:

$$\psi_1 = 2H_p(f_0), \quad \psi_2(f) = 2H_p(f),$$

where $H_p = D_p^\top D_p$ for $D_p : f \to \frac{\partial}{\partial x_p} f$ the differentiation operator and $D_p^\top$ the adjoint of $D_p$. Given data $\{\mathbf{x}_i, y_i\}_{i=1}^n$, recall the definition of $\mathbf{\Phi}$, $\partial_p\mathbf{\Phi}$ (Section A) and denote $\mathbf{\Phi}^+_{K\times n}$ the generalized inverse of $\mathbf{\Phi}$, the operator $D_p$ can be evaluated in matrix form as $\mathbf{D}_p = \partial_p\mathbf{\Phi}\mathbf{\Phi}^+$, and $D_p(f)$ can be evaluated as $\mathbf{D}_p\mathbf{f} = (\partial_p\mathbf{\Phi}\mathbf{\Phi}^+)\mathbf{\Phi}\boldsymbol{\beta} = \partial_p\mathbf{\Phi}\boldsymbol{\beta}$ for $f \in \mathcal{F}(L, K, S, B)$. Correspondingly, the operator $H_p$ adopts matrix reprentation $\mathbf{H}_p = \mathbf{D}_p^\top\mathbf{D}_p = (\mathbf{\Phi}^+)^\top\partial_p\mathbf{\Phi}^\top\partial_p\mathbf{\Phi}\mathbf{\Phi}^+$, such that $\langle H_p(f), f\rangle = (\mathbf{H}_p\mathbf{\Phi}\boldsymbol{\beta})^\top\mathbf{\Phi}\boldsymbol{\beta} = (\partial_p\mathbf{\Phi}\boldsymbol{\beta})^\top(\partial_p\mathbf{\Phi}\boldsymbol{\beta})$.

Finally, for the decomposition $W_n(f) = \langle \omega, f\rangle_n + \Delta_n(f)$, we will define $\omega = P_{\mathcal{F}}(\epsilon)$ the projection of $\epsilon$ to $\mathcal{F}$, and $\Delta_n(f) = \langle P_{\mathcal{F}}^\perp(\epsilon), f\rangle$. Given observations $\{\mathbf{x}_i, y_i\}_{i=1}^n$, the projection operator $P_{\mathcal{F}}^\perp$ can be evaluated by computing the projection matrix $\mathbf{P}_{\mathcal{F}} = \mathbf{U}\mathbf{U}^\top$ and $\mathbf{P}_{\mathcal{F}}^\perp = \mathbf{I} - \mathbf{U}\mathbf{U}^\top$ for

$\mathbf{\Phi}_{n\times K} = \mathbf{U}_{n\times K}\mathbf{D}_{K\times K}\mathbf{V}^\top_{K\times K}$. By noticing that $\mathbf{P}_\mathcal{F}$ is a rank $K$ matrix, it is then easy to see that the two conditions (6) and (7) are satisfied since $||\omega||_n = O(K) \lesssim O(\sqrt{n})$ and $P^\perp_\mathcal{F}(\epsilon)$ is orthogonal to $\psi_2(f - f_0) \in \mathcal{F}_\mathcal{W}$.

As an aside, we note that due to the existence of the bias term at the output layer, the actual feature matrix is $\mathbf{\Phi}_1 = [\mathbf{1}, \mathbf{\Phi}]$. However, this does not impact the expression of $\mathbf{D}_p$ or $\mathbf{H}_p$, since $\mathbf{D}_p = \partial_p\mathbf{\Phi}_1\mathbf{\Phi}_1^+ = [\mathbf{0}, \partial_p\mathbf{\Phi}][(\mathbf{1}^+)^\top, (\mathbf{\Phi}^+)^\top]^\top = \partial_p\mathbf{\Phi}\mathbf{\Phi}^+$ where $\mathbf{1}^+_{n\times 1}$ is a vector that is orthogonal to $\mathbf{1}_{n\times 1}$ and $\mathbf{\Phi}^+_{n\times K}$.

### Multivariate Case

Now we consider the multivariate case for $\psi(f) = [||\frac{\partial}{\partial x_1}f||^2_n, \dots, ||\frac{\partial}{\partial x_P}f||^2_n]^\top$ by changing $\psi_1$ and $\psi_2$ to their multivariate counterparts. Specifically, define the operator $H$:

$$H(f) = [H_1(f), \dots, H_P(f)]^\top,$$

where $H_p = D_p^\top D_p$ for $D_p : f \to \frac{\partial}{\partial x_p}f$, so that the functional of interest $\psi^c(f)$ can still be expressed as $\psi^c(f) = \langle H(f), f\rangle_n - E\big(\langle H(\omega), \omega\rangle_n\big)$.

Now verify (5) the smoothness condition for functional of interest $\psi(f)$ and derive expressions for $\psi_1, \psi_2$. The centered quadratic norm of gradient $\psi^c(f)$ adopts the smoothness expansion:

$$\psi(f) - \psi(f_0) = \langle \psi_1, f - f_0\rangle_n + \frac{1}{2}\langle \psi_2(f - f_0), f - f_0\rangle_n + o_p(\sqrt{n})$$

in which $\psi_1$ and $\psi_2$ are two $P \times 1$ vectors that take the form:

$$\psi_1 = 2H(f_0), \quad \psi_2(f) = 2H(f)$$

Given data $\{\mathbf{x}_i, y_i\}_{i=1}^n$, recall that the operator $D_p$ can be evaluated in matrix form as $\mathbf{D}_p = \partial_p\mathbf{\Phi}\mathbf{\Phi}^+$ and $H_p$ can be evaluated as $\mathbf{H}_p = \mathbf{D}_p^\top\mathbf{D}_p = \mathbf{\Phi}^{+\top}\partial_p\mathbf{\Phi}^\top\partial_p\mathbf{\Phi}\mathbf{\Phi}^+$. Correspondingly, $H(f)$ adopts matrix reprentation $\mathbf{Hf}_{n\times P} = [(\mathbf{H}_1\mathbf{f})_{n\times 1}, \dots, (\mathbf{H}_P\mathbf{f})_{n\times 1}] = [\mathbf{\Phi}^{+\top}\partial_1\mathbf{\Phi}^\top\partial_1\mathbf{\Phi}\boldsymbol{\beta}, \dots, \mathbf{\Phi}^{+\top}\partial_P\mathbf{\Phi}^\top\partial_P\mathbf{\Phi}\boldsymbol{\beta}]$, such that $\langle H_p(f), f\rangle_n$ is evaluated as $\psi_{P\times 1} = (\mathbf{Hf}_{n\times P})^\top\mathbf{f}_{n\times 1} = \big[||\partial_1\mathbf{\Phi}\boldsymbol{\beta}||^2_2, \dots, ||\partial_P\mathbf{\Phi}\boldsymbol{\beta}||^2_2\big]^\top$.

## C.3 Preliminary II: Proof Strategy and Preliminary Theorems

Recall that under a deep ReLU neural network, the prior distribution adopts a conditional Gaussian process representation (Section A.3):

$$\Pi(f, \mathcal{W}) = \Pi(f|\mathcal{W})\Pi(\mathcal{W}) = GP(f|0, k_\mathcal{W})\Pi(\mathcal{W}).$$

This decomposition suggests that a neural network model can be treated as a Gaussian process with an adaptive kernel function $k_\mathcal{W}$, whose hyperparameters $\mathcal{W}$ follows a prior distribution $\Pi(\mathcal{W})$.

Consequently, we use a two-step strategy to show BvM phenomenon for ReLU network:

- **Step 1**, fix hidden weight $\mathcal{W}$ and show BvM phenonmenon hold for $GP(f|0, k_\mathcal{W})$. This essentially corresponding to performing Bayesian inference for a *randomized neural network* whose hidden weights are sampled *a priori* from certain fixed distribution [15]. Then
- **Step 2**, we show that such BvM phenonmenon for $\Pi_n(f|\mathcal{W})$ still holds under the posterior distribution of hidden weights $\mathcal{W} \sim \Pi_n(\mathcal{W})$.

Theorem C.2 establishes **Step 1**. Notice that in the fixed-$\mathcal{W}$ case, $f \in \mathcal{F}$ follows an exact GP with effective model dimension $K$ (i.e. the rank of the kernel matrix), for whom the BvM phenonmenon are known to hold under suitable regularity conditions [5, 6]. Therefore it is expected that BvM to hold for randomized neural network $f \in \mathcal{F}_\mathcal{W}$, provided $K$ does not grow too fast with respect to $n$ (i.e. Assumption (1)) and the functional $\psi_p(f)$ is sufficiently smooth (i.e. satisfying (5)), which is true for $\psi_p(f) = ||\frac{\partial}{\partial x_p}f||^2_n$:

**Theorem C.2** (Bernstein-von Mises (BvM) for $\psi^c_p$, Fixed Hidden Weights)**.** *For $f \in \mathcal{F}_\mathcal{W}(L, W, S, B)$ a deep ReLU network with hidden weight fixed to $\mathcal{W}$, denoting $f_{0,\mathcal{W}}$ the projection of $f_0$ to $\mathcal{F}_\mathcal{W}$, and assume the posterior distribution $\Pi_n(f|\mathcal{W})$ contracts around $f_{0,\mathcal{W}}$ at rate*

*$\epsilon_n$. Denote $D_{\mathcal{W},p} : f \to \frac{\partial}{\partial x_p} f$ the differentiation operator in $\mathcal{F}_{\mathcal{W}}$, and $H_{\mathcal{W},p} = D_{\mathcal{W},p}^\top D_{\mathcal{W},p}$ the corresponding self-adjoint operator. For $\omega_{\mathcal{W}} = Proj_{\mathcal{F}_{\mathcal{W}}}(\boldsymbol{\epsilon})$ the projection of $\epsilon$ to $\mathcal{F}_{\mathcal{W}}$, define:*

$$\hat{\psi}_{\mathcal{W},p} = ||D_{\mathcal{W},p}(f_0 + \omega_{\mathcal{W}})||_n^2 = \psi_{\mathcal{W},p}(f_{0,\mathcal{W}}) + 2\langle H_{\mathcal{W},p} f_{0,\mathcal{W}}, \omega_{\mathcal{W}}\rangle_n + \langle H_{\mathcal{W},p}\omega_{\mathcal{W}}, \omega_{\mathcal{W}}\rangle_n, \quad (10)$$

*Define $\hat{\psi}^c_{\mathcal{W},p} = \hat{\psi}_{\mathcal{W},p} - \hat{\eta}_{\mathcal{W},n}$ where $\hat{\eta}_{\mathcal{W},n} = tr\big(\widehat{H}_{\mathcal{W},p}\big)/n$. Then $\hat{\psi}^c_{\mathcal{W},p}$ is an unbiased estimator of $\psi_{\mathcal{W},p}(f_0)$, and the posterior distribution for $\psi^c_{\mathcal{W},p}(f)$ is asymptotically normal surrounding $\hat{\psi}^c_{\mathcal{W},p}$, i.e.*

$$\Pi\Big(\sqrt{n}(\psi^c_{\mathcal{W},p}(f) - \hat{\psi}^c_{\mathcal{W},p})\Big|\{\mathbf{x}_i, y_i\}_{i=1}^n, \mathcal{W}\Big) \rightsquigarrow N(0, 4||H_{\mathcal{W},p} f_{0,\mathcal{W}}||_n^2), \quad (11)$$

The proof is delayed to Section D.1. It should be stressed that both operators $D_{\mathcal{W},p}$ and $H_{\mathcal{W},p}$ are defined strictly with respect to $\mathcal{F}_{\mathcal{W}}$. Such that given data, the operator $D_{\mathcal{W},p}$ is estimated in matrix form as $\widehat{\mathbf{D}}_{\mathcal{W},p} = \partial_p \mathbf{\Phi}_{\mathcal{W}} \mathbf{\Phi}^+_{\mathcal{W}}$, and $H_{\mathcal{W},p}$ is evaluated as $\widehat{\mathbf{H}}_{\mathcal{W},p} = (\mathbf{\Phi}^+_{\mathcal{W}})^\top \partial_p \mathbf{\Phi}^\top_{\mathcal{W}} \partial_p \mathbf{\Phi}_{\mathcal{W}} \mathbf{\Phi}^+_{\mathcal{W}}$. In comparison, the original $D_p$ and $H_p$ defined Section C.2 are with respect to the optimal solution $f_0 \in \mathcal{F}$.

### C.4 Proof for Theorem 2

We now prove Theorem 2, which establishes **Step 2** of the proof strategy outlined in Section C.3.

Our goal is to show that the BvM phenomenon in Theorem C.2 still holds under the *adaptive* case (i.e. $\mathcal{W}$ is not fixed but follows the posterior distribution $\Pi_n(\mathcal{W})$), and furthermore, the whole posterior distribution of $\sqrt{n}(\psi^c_p(f) - \hat{\psi}^c_p(f))$ converges to $N(0, 4||H_p f_0||_n^2)$ where $H_p$ is defined with respect to the optimal solution $f_0 \in \mathcal{F}$.

*Proof.* Our goal is to show:

$$\Pi\Big(\sqrt{n}(\psi^c_p(f) - \hat{\psi}^c_p)\Big|\{\mathbf{x}_i, y_i\}_{i=1}^n\Big) \rightsquigarrow N(0, 4||H_p f_0||_n^2).$$

First notice that by Theorem C.2, the asymptotic distribution of the marginal posterior distribution can be represented as a mixture of Gaussian:

$$\begin{aligned}
\Pi_n\Big(\sqrt{n}(\psi^c_p(f) - \hat{\psi}^c_p) \leq z\Big) &= \int_{\mathcal{W}} \Pi_n\Big(\sqrt{n}(\psi^c_p(f) - \hat{\psi}^c_p) \leq z|\mathcal{W}\Big) d\Pi_n(\mathcal{W}) \\
&= \int_{\mathcal{W}} \Pi_n\Big(\sqrt{n}(\psi^c_p(f) - \hat{\psi}^c_{\mathcal{W},p}) \leq z + \sqrt{n}(\hat{\psi}^c_p - \hat{\psi}^c_{\mathcal{W},p})|\mathcal{W}\Big) d\Pi_n(\mathcal{W}) \\
&= \int_{\mathcal{W}} \Phi\Big(\big(z + \sqrt{n}(\hat{\psi}^c_p - \hat{\psi}^c_{\mathcal{W},p})\big)/\sqrt{V_{\mathcal{W},0}}\ |\mathcal{W}\Big) d\Pi_n(\mathcal{W}) \quad (12)
\end{aligned}$$

where the last line follows from Theorem C.2, where $V_{\mathcal{W},0} = 4||H_{\mathcal{W},p} f_{\mathcal{W},0}||_n^2$ and $\Phi$ is the standard Gaussian cumulative distribution function (CDF).

Clearly, for BvM to hold in the case of (15), it is sufficient to show below two conditions [7]:

$$|V_{\mathcal{W},0} - V_0| = o_p(1), \quad \sqrt{n}|\hat{\psi}^c_p - \hat{\psi}^c_{\mathcal{W},p}| = o_p(1). \quad (13)$$

The first condition follows from the continuous mapping theorem for $V(H_p f_0) = 2||H_p f_0||_n^2$, along with the fact that :

$$\begin{aligned}
||H_{\mathcal{W},p} f_{\mathcal{W},0} - H_p f_0||_n &\leq ||(H_{\mathcal{W},p} - H_p) f_0||_n + ||H_{\mathcal{W},p}(f_{\mathcal{W},0} - f_0)||_n \\
&= O(||H_{\mathcal{W},p} - H_p||_n) + O(||f_{\mathcal{W},0} - f_0||_n), \\
&= O(\frac{1}{\sqrt{n}}||H_{\mathcal{W},p} - H_p||_F) + o_p(1) \\
&= O(\frac{K}{\sqrt{n}}) + o_p(1) = o_p(1),
\end{aligned}$$

where the first equality follows from the boundedness of $\|f_0\|_\infty$ and $\|H_{\mathcal{W},p}\|_\infty$ (by assumption in main article and also Proposition 2), the second equality follows from the definition of $||.||_n$ for matrix and the fact about posterior concentration of $||f - f_0||_n^2$ in the statement of Theorem 2. The last line follows since $||\mathbf{H}_p||_F = O(K)$ by Proposition (2) and the assumption that $K = o_p(\sqrt{n})$ (Assumption (1) in the main article).

The second condition in (13) is the important *no-bias* condition which ensures that under $\mathcal{W} \sim \Pi_n(\mathcal{W})$, all the conditional posterior $\psi_p^c|\mathcal{W}$ converges toward the same target $\hat{\psi}_p^c$ [7, 19]. Recall that $\hat{\psi}_p^c = \psi_p(f_0) + 2\langle H_p f_0, \omega\rangle_n + \langle H_p\omega, \omega\rangle_n - E(\langle H_p\omega, \omega\rangle_n)$, then the second condition can be written as:

$$\sqrt{n}|\hat{\psi}_p^c - \hat{\psi}_{\mathcal{W},p}^c| \leq \sqrt{n}|\psi_p(f_0) - \psi_{\mathcal{W},p}(f_{\mathcal{W},0})| + 2\sqrt{n}|\langle H_p f_0, \omega\rangle_n - \langle H_{\mathcal{W},p} f_{\mathcal{W},0}, \omega_{\mathcal{W}}\rangle_n| + \sqrt{n}|\langle H_{\mathcal{W},p}\omega_{\mathcal{W}}, \omega_{\mathcal{W}}\rangle_n - \langle H_p\omega, \omega\rangle_n| + \sqrt{n}|E(\langle H_{\mathcal{W},p}\omega_{\mathcal{W}}, \omega_{\mathcal{W}}\rangle_n) - E(\langle H_p\omega, \omega\rangle_n)|, \tag{14}$$

where all four terms are $o_p(1)$ since they are all $O_p(K/\sqrt{n})$ and the model dimension $K$ is by assumption not too large (i.e. $K = o(n^{1/2})$). We delay the detailed arguments to the end of the proof.

Consequently, since both conditions in (13) are satisfied, the expression in (15) converge uniquely to a normal distribution under the posterior distribution $\Pi_n(\mathcal{W})$, i.e.,

$$\begin{aligned}\Pi_n\Big(\sqrt{n}(\psi_p^c(f) - \hat{\psi}_p^c) \leq z\Big) &= \int_{\mathcal{W}} \Phi\Big(\big(z + \sqrt{n}(\hat{\psi}_p^c - \hat{\psi}_{\mathcal{W},p}^c)\big)/\sqrt{V_{\mathcal{W},0}}\ \big|\mathcal{W}\Big) d\Pi_n(\mathcal{W}) \\ &= \int_{\mathcal{W}} \Phi\Big(\big(z + o_p(1)\big)/\sqrt{V_0 + o_p(1)}\ \big|\mathcal{W}\Big) d\Pi_n(\mathcal{W}) \\ &= \Phi\big(z/\sqrt{V_0}\big), \qquad \text{where} \qquad V_0 = 4||H_0 f_0||_n^2 \end{aligned} \tag{15}$$

which implies the statement of interest:

$$\Pi\Big(\sqrt{n}(\psi_p^c(f) - \hat{\psi}_p^c)\Big|\{\mathbf{x}_i, y_i\}_{i=1}^n\Big) \rightsquigarrow N(0, 4||H_p f_0||_n^2).$$

We are only left to show that all four terms in the expression (14) are $o_p(1)$. Specifically, recall that $H_p = D_p^\top D_p$ such that $\langle H_p a, b\rangle_n = \langle D_p a, D_p b\rangle_n$ for any $a, b \in \mathcal{F}$, then:

- **First Term**: Recall $\psi_p(f_0) = \langle H_p f_0, f_0\rangle_n = ||D_p f_0||_n^2$, then the first term can be expressed as:

$$\begin{aligned}\sqrt{n}|\psi_p(f_0) - \psi_{\mathcal{W},p}(f_{\mathcal{W},0})| &= \sqrt{n}\Big|||D_p f_0||_n^2 - ||D_{\mathcal{W},p} f_{\mathcal{W},0}||_n^2\Big| \\ &\leq \sqrt{n}\Big(||D_p||_n^2||f_0||_n^2 + ||D_{\mathcal{W},p}||_n^2||f_{\mathcal{W},0}||_n^2\Big) \\ &= \sqrt{n}\Big(O_p(||D_p||_n^2) + O_p(||D_{\mathcal{W},p}||_n^2)\Big) = \frac{1}{\sqrt{n}}\Big(O_p(||\mathbf{D}_p||_F^2) + O_p(||\mathbf{D}_{\mathcal{W},p}||_n^2)\Big) \\ &= O(\frac{K}{\sqrt{n}}) = o_p(1)\end{aligned}$$

  where on the third line, the first equality follows since $f_0$ and $f_{\mathcal{W},0}$ are both bounded, the second equality follows by the definition of the matrix Euclidean norm $||\mathbf{M}||_n^2 = \frac{1}{n}\sum_{i,j}\mathbf{M}_{i,j}^2 = \frac{1}{n}||\mathbf{M}||_F^2$. On the last line, the first eqality follows by $||\mathbf{D}_{\mathcal{W},p}||_F^2 = tr(\mathbf{H}_{\mathcal{W},p}) = O(K)$ due to Proposition 2, and the second equality follows by Assumption $K = o_p(n^{1/2})$.

- **Second Term**: Similarly, the second term can be expressed as:

$$\begin{aligned}\sqrt{n}|\langle H_p f_0, \omega\rangle_n - \langle H_{\mathcal{W},p} f_{\mathcal{W},0}, \omega_{\mathcal{W}}\rangle_n| &= \sqrt{n}\big|\langle D_p f_0, D_p\omega\rangle_n - \langle D_{\mathcal{W},p} f_{\mathcal{W},0}, D_{\mathcal{W},p}\omega_{\mathcal{W}}\rangle_n\big| \\ &\leq \sqrt{n}\Big(||D_p||_n^2||f_0||_n||\omega||_n + ||D_{\mathcal{W},p}||_n^2||f_{\mathcal{W},0}||_n||\omega_{\mathcal{W}}||_n\Big) \\ &= \sqrt{n}\Big(O_p(||D_p||_n^2) + O_p(||D_{\mathcal{W},p}||_n^2)\Big) \\ &= O_p(\frac{K}{\sqrt{n}}) = o_p(1)\end{aligned}$$

where the equality on the third line follows from the fact that $f_{0,\mathcal{W}}$ is bounded and $\omega = P_{\mathcal{F}}\epsilon$ is a random variable with bounded variance. The rest of the equalities follow similarly as those in the First term.

- **Third and Fourth Terms** are similar to the first term except for $f_0$ is replaced by $\omega$. As a result:

$$\begin{aligned}
\sqrt{n}|\langle H_{\mathcal{W},p}\omega_{\mathcal{W}}, \omega_{\mathcal{W}}\rangle_n - \langle H_p\omega, \omega\rangle_n| &= \sqrt{n}\Big|||D_{\mathcal{W},p}\omega_{\mathcal{W}}||_n^2 - ||D_p\omega||_n^2\Big| \\
&= \sqrt{n}\Big(O_p(||D_p||_n^2) + O_p(||D_{\mathcal{W},p}||_n^2)\Big) \\
&= O_p(\frac{K}{\sqrt{n}}) = o_p(1) \\
\sqrt{n}|E(\langle H_{\mathcal{W},p}\omega_{\mathcal{W}}, \omega_{\mathcal{W}}\rangle_n) - E(\langle H_p\omega, \omega\rangle_n)| &= \sqrt{n}O_p\Big(|\langle H_{\mathcal{W},p}\omega_{\mathcal{W}}, \omega_{\mathcal{W}}\rangle_n - \langle H_p\omega, \omega\rangle_n|\Big) \\
&= O_p(\frac{K}{\sqrt{n}}) = o_p(1)
\end{aligned}$$

□

### C.5 Proof for Theorem 3

To prepare for the multivariate BvM theorem (Theorem 3), below theorem extends Theorem C.2 to the multivariate case for $\psi(f) = [||\frac{\partial}{\partial x_1}f||_n^2, \dots, ||\frac{\partial}{\partial x_p}f||_n^2]^\top$.

**Theorem C.3** (Multivariate BvM for $\psi^c$, Fixed Hidden Weights). *For $f \in \mathcal{F}_{\mathcal{W}}(L, W, S, B)$, assuming the posterior distribution $\Pi_n(f)$ contracts around $f_{0,\mathcal{W}}$ at rate $\epsilon_n$. For $\omega_{\mathcal{W}} = Proj_{\mathcal{F}_{\mathcal{W}}}(\boldsymbol{\epsilon})$, denote $\hat{\psi}^c_{\mathcal{W}} = [\hat{\psi}^c_{\mathcal{W},1}, \dots, \hat{\psi}^c_{\mathcal{W},P}]$ for $\hat{\psi}^c_{\mathcal{W},p}$ as defined in Theorem C.2.*

*Then $\hat{\psi}^c_{\mathcal{W}}$ is an unbiased and efficient estimator of $\psi_{\mathcal{W}}(f_0)$, and the posterior distribution for $\psi^c_{\mathcal{W}}(f)$ asymptotically converge toward a multivariate normal distribution surrounding $\hat{\psi}^c_{\mathcal{W}}$, i.e.*

$$\Pi\Big(\sqrt{n}(\psi^c_{\mathcal{W}}(f) - \hat{\psi}^c_{\mathcal{W}})\Big|\{\mathbf{x}_i, y_i\}_{i=1}^n\Big) \rightsquigarrow MVN(0, V_{0,\mathcal{W}}), \tag{16}$$

*where $V_{0,\mathcal{W}}$ is a $P \times P$ matrix such that $(V_{0,\mathcal{W}})_{p_1,p_2} = 4\langle H_{\mathcal{W},p_1}f_{0,\mathcal{W}}, H_{\mathcal{W},p_2}f_{0,\mathcal{W}}\rangle_n$.*

The proof is in Section D.2. We are now ready to prove Theorem 3.

*Proof.* Our goal is to show:

$$\Pi\Big(\sqrt{n}(\psi^c(f) - \hat{\psi}^c)\Big|\{\mathbf{x}_i, y_i\}_{i=1}^n\Big) \rightsquigarrow N(0, V_0). \tag{17}$$

We show the convergence of above multivariate normal distribution by involing the Cramér-Wold device, i.e. we show that for all $t \in \mathbb{R}^P$:

$$\Pi\Big(\sqrt{n}\,(t^\top\psi^c(f) - t^\top\hat{\psi}^c)\Big|\{\mathbf{x}_i, y_i\}_{i=1}^n\Big) \rightsquigarrow N(0, t^\top V_0 t).$$

Similar to the scalar case, the asymptotic distribution of the marginal posterior distribution can be represented as a mixture of Gaussian:

$$\begin{aligned}
\Pi_n\Big(\sqrt{n}(t^\top\psi^c(f) - t^\top\hat{\psi}^c) \le z\Big) &= \int_{\mathcal{W}} \Pi_n\Big(t^\top\sqrt{n}(\psi^c(f) - t^\top\hat{\psi}^c_p) \le z|\mathcal{W}\Big)d\Pi_n(\mathcal{W}) \\
&= \int_{\mathcal{W}} \Pi_n\Big(\sqrt{n}(t^\top\psi^c(f) - t^\top\hat{\psi}^c_{\mathcal{W},p}) \le z + \sqrt{n}(t^\top\hat{\psi}^c_p - t^\top\hat{\psi}^c_{\mathcal{W},p})|\mathcal{W}\Big)d\Pi_n(\mathcal{W}) \\
&= \int_{\mathcal{W}} \Phi\Big(\big(z + \sqrt{n}(t^\top\hat{\psi}^c_p - t^\top\hat{\psi}^c_{\mathcal{W},p})\big)/\sqrt{t^\top V_{\mathcal{W},0}t}\;|\mathcal{W}\Big)d\Pi_n(\mathcal{W})
\end{aligned} \tag{18}$$

where the last line follows from Theorem C.3, where $(V_{0,\mathcal{W}})_{p_1,p_2} = 4\langle H_{\mathcal{W},p_1}f_{0,\mathcal{W}}, H_{\mathcal{W},p_2}f_{0,\mathcal{W}}\rangle_n$ and $\Phi$ is the standard Gaussian CDF.

Therefore it is sufficient to show below two conditions [7]:

$$t^\top (V_{\mathcal{W},0} - V_0)t = o_p(1), \quad \sqrt{n}|t^\top \hat{\psi}^c - t^\top \hat{\psi}^c_{\mathcal{W}}| = o_p(1). \tag{19}$$

However, both conditions follows from the coordinate-wise convergence $\sqrt{n}|\hat{\psi}^c_p - \hat{\psi}^c_{\mathcal{W},p}| = o_p(1)$ and $||H_{\mathcal{W},p} f_{\mathcal{W},0} - H_p f_0||_n = o_p(1)$, which were established in the proof for Theorem 2.

Consequently, the expression in (18) converge uniquely to a normal distribution under the posterior distribution $\Pi_n(\mathcal{W})$, i.e.,

$$\begin{aligned}\Pi_n\Big(\sqrt{n}(t^\top \psi^c(f) - t^\top \hat{\psi}^c) \leq z\Big) &= \int_{\mathcal{W}} \Phi\Big(\big(z + \sqrt{n}(t^\top \hat{\psi}^c_p - t^\top \hat{\psi}^c_{\mathcal{W},p})\big)/\sqrt{t^\top V_{\mathcal{W},0} t}\;\big|\mathcal{W}\Big) d\Pi_n(\mathcal{W}) \\ &= \int_{\mathcal{W}} \Phi\Big(\big(z + o_p(1)\big)/\sqrt{t^\top V_0 t + o_p(1)}\;\big|\mathcal{W}\Big) d\Pi_n(\mathcal{W}) \\ &= \Phi\big(z/\sqrt{t^\top V_0 t}\big), \qquad \text{where} \qquad (V_0)_{p_1,p_2} = 4\langle H_{p_1} f_0, H_{p_2} f_0\rangle_n\end{aligned}$$

which implies the statement of interest (17).

□

# D Additional Proofs

## D.1 Proof for Theorem C.2

*Proof.* Our goal is to show asymptotic normality

$$\Pi_n\big(\sqrt{n}(\psi^c_{\mathcal{W},p}(f) - \hat{\psi}^c_{\mathcal{W},p})|\mathcal{W}\big) \rightsquigarrow N(0, ||\psi_1||_n^2).$$

First derive the expressions for $f_t, \hat{\psi}_{\mathcal{W},p}, V_{0,n}$ and $\mathcal{I}_n$. The expression for $f_t$ is:

$$\begin{aligned} f_t &= f - \frac{t}{\sqrt{n}}\Big(\psi_1 + \frac{1}{2}\psi_2(f - f_{0,\mathcal{W}})\Big) - \frac{t}{2n}\psi_2(\omega_{\mathcal{W}}) \\ &= \Big(I - \frac{t}{\sqrt{n}} * H_p\Big)(f) - \frac{t}{\sqrt{n}} * H_p\big(f_{0,\mathcal{W}} + \omega_{\mathcal{W}}\big). \end{aligned} \tag{20}$$

where $I : f \to f$ is the identity operator. The expressions for $\hat{\psi}_{\mathcal{W},p}$ and $V_{0,n}$ are (recall $\omega_{\mathcal{W}} = P_{\mathcal{F}_{\mathcal{W}}}(\epsilon)$):

$$\begin{aligned} \hat{\psi}_{\mathcal{W},p} &= \psi_{\mathcal{W},p}(f_{0,\mathcal{W}}) + \frac{W_n(\psi_1)}{\sqrt{n}} + \frac{1}{2}\frac{\langle\omega_{\mathcal{W}}, \psi_2(\omega_{\mathcal{W}})\rangle_n}{n} \\ &= \psi_{\mathcal{W},p}(f_{0,\mathcal{W}}) + 2\langle H_{\mathcal{W},p}f_{0,\mathcal{W}}, \omega_{\mathcal{W}}\rangle_n + \langle H_{\mathcal{W},p}\omega_{\mathcal{W}}, \omega_{\mathcal{W}}\rangle_n, \\ V_{0,n} &= \Big|\Big|\psi_1 - \frac{1}{2}\frac{\psi_2(\omega_{\mathcal{W}})}{\sqrt{n}}\Big|\Big|_n^2 = 4 * \Big|\Big|H_{\mathcal{W},p}f_{0,\mathcal{W}} + o_p(1)\Big|\Big|_n^2, \end{aligned}$$

and the expression for $\mathcal{I}_n$ is:

$$\mathcal{I}_n = \frac{\int_{A_n} e^{l_n(f_t) - l_n(f_{0,\mathcal{W}})} d\Pi(f|\mathcal{W})}{\int_{A_n} e^{l_n(f) - l_n(f_{0,\mathcal{W}})} d\Pi(f|\mathcal{W})}.$$

It then follows from the Theorem C.1 that

$$E_n(e^{t\sqrt{n}(\psi^c_{\mathcal{W},p}(f) - \hat{\psi}^c_{\mathcal{W},p})}|A_n, \mathcal{W}) = e^{o_p(1) + t^2 V_{0,n}/2} * \mathcal{I}_n. \tag{21}$$

Therefore to show asymptotic normality $\Pi_n\big(\sqrt{n}(\psi^c_{\mathcal{W},p}(f) - \hat{\psi}^c_{\mathcal{W},p})|\mathcal{W}\big) \rightsquigarrow N(0, ||\psi_1||_n^2)$, we only need to show $\mathcal{I}_n \to 1$ for some suitable choice of $A_n$ so that $E_n(e^{t\sqrt{n}(\psi^c_{\mathcal{W},p}(f) - \hat{\psi}^c_{\mathcal{W},p})}|A_n, \mathcal{W}) \to e^{t^2 V_0/2}$. To this end, we consider the standard choice $A_n = \Big\{f \Big| ||f - f_{0,\mathcal{W}}||_n^2 \leq M_n \epsilon_n\Big\}$ for some sufficiently large $M_n \to \infty$ and $\epsilon_n$ the given rate of posterior convergence.

To analyze the asymptotic behavior of $\mathcal{I}_n$, analogous to the Theorem 3.1 of [7], we consider the asymptotically equivalent term $\mathcal{I}'_n$:

$$\mathcal{I}'_n = \frac{\int_{f \in A_n} e^{l_n(f_t) - l_n(f_{0,\mathcal{W}})} d\Pi(f|\mathcal{W})}{\int e^{l_n(f) - l_n(f_{0,\mathcal{W}})} d\Pi(f|\mathcal{W})}$$

where the denominator $\int_{A_n}$ in $\mathcal{I}_n$ is replaced by $\int$. $\mathcal{I}'_n$ is asymptotically equivalent to $\mathcal{I}_n$ since $\Pi_n(A_n) = 1 + o_p(1)$.

Notice that $\mathcal{I}'_n$ can be written as:

$$\mathcal{I}'_n = \mathcal{J}_n * \mathcal{K}_n = \frac{\int e^{l_n(f_t) - l_n(f_{0,\mathcal{W}})} d\Pi(f|\mathcal{W})}{\int e^{l_n(f) - l_n(f_{0,\mathcal{W}})} d\Pi(f|\mathcal{W})} * \frac{\int_{f \in A_n} e^{l_n(f_t) - l_n(f_{0,\mathcal{W}})} d\Pi(f|\mathcal{W})}{\int e^{l_n(f_t) - l_n(f_{0,\mathcal{W}})} d\Pi(f|\mathcal{W})}$$

where we have denoted:

$$\mathcal{J}_n = \frac{\int e^{l_n(f_t) - l_n(f_{0,\mathcal{W}})} d\Pi(f|\mathcal{W})}{\int e^{l_n(f) - l_n(f_{0,\mathcal{W}})} d\Pi(f|\mathcal{W})}, \quad \mathcal{K}_n = \frac{\int_{f \in A_n} e^{l_n(f_t) - l_n(f_{0,\mathcal{W}})} d\Pi(f|\mathcal{W})}{\int e^{l_n(f_t) - l_n(f_{0,\mathcal{W}})} d\Pi(f|\mathcal{W})}. \tag{22}$$

Therefore in order to show $\mathcal{I}_n \to 1$, it is sufficient to show $\mathcal{J}_n \to 1$ and $\mathcal{K}_n \to 1$.

We show $\mathcal{J}_n \to 1$ by first performing change of variables $f \to f_t$ on the numerator, and then analyze the asymptotic behavior of the resulting expression. To this end, notice that the conditional prior

$\Pi(f|\mathcal{W})$ is a Gaussian process prior with kernel function $k_{\mathcal{W}}(\mathbf{x}, \mathbf{x}') = \sum_{k=1}^{K} \phi_k(\mathbf{x}|\mathcal{W})\phi_k(\mathbf{x}'|\mathcal{W}) + \sigma_{b_0}^2$, and correspondingly, the kernel matrix evaluated at $\{\mathbf{x}_i, y_i\}_{i=1}^n$ is $\mathbf{K}_{\mathcal{W}} = \mathbf{\Phi}_{\mathcal{W}}\mathbf{\Phi}_{\mathcal{W}}^\top + \sigma_{b_0}^2\mathbf{I}$ for $\mathbf{\Phi}_{n\times K} = \mathbf{X}(\prod_{l=1}^{L}\mathbf{W}_l\mathbf{S}_l)$ (see Section A.1). Therefore given observations $\{y_i, \mathbf{x}_i\}_{i=1}^n$, the conditional prior distribution for $\mathbf{f} = [f(\mathbf{x}_1), \dots, f(\mathbf{x}_n)]^\top \in \mathbb{R}^n$ is a multivariate Gaussian with covariance matrix $\mathbf{K}_{\mathcal{W}}$:

$$d\Pi(\mathbf{f}|\mathcal{W}) \propto |\mathbf{K}_{\mathcal{W}}|^{-\frac{1}{2}} e^{-\frac{1}{2}\mathbf{f}^\top\mathbf{K}_{\mathcal{W}}^{-1}\mathbf{f}}$$

where $|\mathbf{K}_{\mathcal{W}}|$, $\mathbf{K}_{\mathcal{W}}^{-1}$ are the determinant and inverse of $\mathbf{K}_{\mathcal{W}}$, respectively. To perform change of variable, we denote $\mathbf{f}_t \in \mathbb{R}^n$ as $f_t$ in (20) evaluated at $\{y_i, \mathbf{x}_i\}_{i=1}^n$, we can write $\mathbf{f}_t = \mathbf{B}_{t,n}\mathbf{f} - \frac{t}{\sqrt{n}}\mathbf{a}_n$ such that

$$\begin{aligned} d\Pi(\mathbf{f}_t|\mathcal{W}) &\propto |\mathbf{K}_{n,\mathcal{W}}|^{-\frac{1}{2}} e^{-\frac{1}{2}(\mathbf{f}+\frac{t}{\sqrt{n}}\mathbf{a}_n)^\top\mathbf{K}_{n,\mathcal{W}}^{-1}(\mathbf{f}+\frac{t}{\sqrt{n}}\mathbf{a}_n)} \\ &= d\Pi(\mathbf{f}|\mathcal{W}) * exp\Big[-\frac{1}{2}log\Big(\frac{|\mathbf{K}_{n,\mathcal{W}}|}{|\mathbf{K}_{\mathcal{W}}|}\Big) - \frac{1}{2}\mathbf{f}^\top\big(\mathbf{K}_{n,\mathcal{W}}^{-1} - \mathbf{K}_{\mathcal{W}}^{-1}\big)\mathbf{f} + \frac{t}{\sqrt{n}}\mathbf{a}_n^\top\mathbf{K}_{n,\mathcal{W}}^{-1}\mathbf{f} - \frac{t^2}{2n}\mathbf{a}_n^\top\mathbf{K}_{n,\mathcal{W}}^{-1}\mathbf{a}_n^\top\Big] \end{aligned}$$

where $\mathbf{B}_{t,n} = \mathbf{I} - \frac{t}{\sqrt{n}}\mathbf{H}_p$, $\mathbf{a}_n = \mathbf{H}_p\big(\mathbf{f}_{0,\mathcal{W}} + \omega_{\mathcal{W}}\big)$, and

$$\mathbf{K}_{n,\mathcal{W}} = \mathbf{B}_{t,n}\mathbf{K}_{\mathcal{W}}\mathbf{B}_{t,n} = \mathbf{K}_{\mathcal{W}} - \frac{t}{\sqrt{n}}\Big[\mathbf{K}_{\mathcal{W}}\mathbf{H}_p + \mathbf{H}_p\mathbf{K}_{\mathcal{W}}\mathbf{B}_{t,n}\Big] = \mathbf{K}_{\mathcal{W}} - \frac{t}{\sqrt{n}}d\mathbf{K}_{\mathcal{W}},$$

where we have denoted $d\mathbf{K}_{\mathcal{W}} = \mathbf{K}_{\mathcal{W}}\mathbf{H}_p + \mathbf{H}_p\mathbf{K}_{\mathcal{W}}\mathbf{B}_{t,n}$.

Consequently, the expression of $\mathcal{J}_n$ after the change of variable becomes:

$$\mathcal{J}_n = \frac{\int e^{l_n(f_t)-l_n(f_{0,\mathcal{W}})} * e^{-\mathcal{L}_{t,n}}\, d\Pi(f_t|\mathcal{W})}{\int e^{l_n(f)-l_n(f_{0,\mathcal{W}})}d\Pi(f|\mathcal{W})},$$

where

$$\mathcal{L}_{t,n} = \frac{1}{2}log\Big(\frac{|\mathbf{K}_{n,\mathcal{W}}|}{|\mathbf{K}_{\mathcal{W}}|}\Big) + \frac{1}{2}\mathbf{f}^\top\big(\mathbf{K}_{n,\mathcal{W}}^{-1} - \mathbf{K}_{\mathcal{W}}^{-1}\big)\mathbf{f} - \frac{t}{\sqrt{n}}\mathbf{a}_n^\top\mathbf{K}_{n,\mathcal{W}}^{-1}\mathbf{f} + \frac{t^2}{2n}\mathbf{a}_n^\top\mathbf{K}_{n,\mathcal{W}}^{-1}\mathbf{a}_n^\top. \quad (23)$$

Therefore in order to show $\mathcal{J}_n \to 1$, it is sufficient to show that all terms in $\mathcal{L}_{t,n} = o_p(1)$ are asymptotically vanishing toward zero as $n \to \infty$. We defer the detailed arguements to the end of this proof. If this is true, then it holds that $\mathcal{L}_{t,n} = o_p(1)$ and

$$\mathcal{J}_n = \frac{\int e^{l_n(f_t)-l_n(f_{0,\mathcal{W}})+o_p(1)}\, d\Pi(f_t|\mathcal{W})}{\int e^{l_n(f)-l_n(f_{0,\mathcal{W}})}d\Pi(f|\mathcal{W})} \to 1. \quad (24)$$

We show $\mathcal{K}_n \to 1$ by noticing that $\mathcal{L}_{t,n} = o_p(1)$ implies:

$$\mathcal{K}_n = \frac{\int_{f\in A_n} e^{l_n(f_t)-l_n(f_{0,\mathcal{W}})}\, d\Pi(f|\mathcal{W})}{\int e^{l_n(f_t)-l_n(f_{0,\mathcal{W}})}d\Pi(f|\mathcal{W})} = \frac{\int_{f\in A_n} e^{l_n(f_t)-l_n(f_{0,\mathcal{W}})+o_p(1)}\, d\Pi(f_t|\mathcal{W})}{\int e^{l_n(f_t)-l_n(f_{0,\mathcal{W}})+o_p(1)}d\Pi(f_t|\mathcal{W})}$$

Notice that in the above expression, the event $f \in A_n$ is equivalent to $f_t \in A_{n,t}$ for:

$$\begin{aligned} A_{n,t} &= \Big\{f_t \Big| ||f - f_0||_n^2 \leq M_n\epsilon_n\Big\} \\ &= \Big\{f_t \Big| ||f - f_0||_n^2 \leq M_n\epsilon_n,\ ||f_t - f_0||_n^2 \leq ||f_t - f||_n^2 + ||f - f_0||_n^2\Big\} \\ &\supseteq \Big\{f_t \Big| ||f_t - f_0||_n^2 \leq ||f_t - f||_n^2 + M_n\epsilon_n\Big\} \\ &= \Big\{f_t \Big| ||f_t - f_0||_n^2 \leq O(n^{-1}) + M_n\epsilon_n\Big\} \\ &= \Big\{f_t \Big| ||f_t - f_0||_n^2 \leq M_n'\epsilon_n\Big\} = A_n' \end{aligned}$$

where on the fourth line, the equality follows since $||f_t - f||_n^2 = \frac{1}{n}||\mathbf{f}_t - \mathbf{f}||_2^2 = \frac{t}{\sqrt{n}}||\mathbf{H}_p\mathbf{f} + \mathbf{a}_n||_2^2/n \leq \frac{t}{\sqrt{n}}(||\mathbf{H}_p||_2^2||\mathbf{f}||_2^2/n + ||\mathbf{a}_n||_2^2/n) = O(n^{-\frac{1}{2}})$ since $||\mathbf{H}_p||_2^2 = O_p(1)$ by Proposition 2, and the facts that $||\mathbf{f}||_2^2/n = O_p(1)$ and $||\mathbf{a}_n||_2^2/n = ||\mathbf{H}_p(\mathbf{f}_{0,\mathcal{W}} + \omega_{\mathcal{W}})||^2/n = O_p(1)$ due to boundedness of $\mathbf{f}$,

$\mathbf{f}_0$ and the fact that $\omega_{\mathcal{W}}$ is a random variable with finite variance. Also, on the last line, the equality follows since $n^{-1} \lesssim \epsilon_n$, i.e. the learning rate $\epsilon_n$ is expected to be slower than $O(n^{-1})$. As a result, we see that since the set $A'_n = \Big\{ f \Big| ||f - f_0||_n \leq M'_n \epsilon_n \Big\}$ is of the same form as $A_n$, we have that $\Pi_n(A'_n) \to 1 + o_p(1)$ due to the posterior convergence of $f$ to $f_0$. Consequently:

$$\mathcal{K}_n = \frac{\int_{f_t \in A_{n,t}} e^{l_n(f_t) - l_n(f_{0,\mathcal{W}}) + o_p(1)} \, d\Pi(f_t|\mathcal{W})}{\int e^{l_n(f_t) - l_n(f_{0,\mathcal{W}}) + o_p(1)} d\Pi(f_t|\mathcal{W})} \geq \frac{\int_{f_t \in A'_n} e^{l_n(f_t) - l_n(f_{0,\mathcal{W}}) + o_p(1)} \, d\Pi(f_t|\mathcal{W})}{\int e^{l_n(f_t) - l_n(f_{0,\mathcal{W}}) + o_p(1)} d\Pi(f_t|\mathcal{W})} \to 1 \tag{25}$$

Finally, since we have shown both $\mathcal{J}_n \to 1$ and $\mathcal{K}_n \to 1$, it then follows by Theorem C.1 that the posterior distribution of $\sqrt{n}(\psi^c_{\mathcal{W},p}(f) - \hat{\psi}^c_{\mathcal{W}})$ converge toward a normal law with mean zero and variance $||\psi_1||^2_n = 4||H_{\mathcal{W},p} f_{0,\mathcal{W}}||^2_n$, i.e. we have shown the statement of the interest:

$$\Pi\Big(\sqrt{n}(\psi^c_{\mathcal{W},p}(f) - \hat{\psi}^c_{\mathcal{W}}) \Big| \{\mathbf{x}_i, y_i\}_{i=1}^n, \mathcal{W}\Big) \rightsquigarrow N(0, 4||H_{\mathcal{W},p} f_{0,\mathcal{W}}||^2_n). \tag{26}$$

We are only left to show that $\mathcal{L}_{t,n} = o_p(1)$, i.e. all the four terms in (23) are asymptotically vanishing toward zero. We achieve this by analyzing the asymptotic behavior of the four terms one by one:

- First term: $log\Big(\frac{|\mathbf{K}_{n,\mathcal{W}}|}{|\mathbf{K}_{\mathcal{W}}|}\Big) = log|\mathbf{K}_{n,\mathcal{W}}| - log|\mathbf{K}_{\mathcal{W}}|$

  Performing Taylor Expansion on $log|\mathbf{K}_{n,\mathcal{W}}|$: [1] [2]

$$\begin{aligned} log|\mathbf{K}_{n,\mathcal{W}}| &= log\Big|\mathbf{K}_{\mathcal{W}} - \frac{t}{\sqrt{n}} d\mathbf{K}_{\mathcal{W}}\Big| \\ &= log|\mathbf{K}_{\mathcal{W}}| - \frac{t}{\sqrt{n}} tr(\mathbf{K}^{-1}_{\mathcal{W}} d\mathbf{K}_{\mathcal{W}}) + \frac{t^2}{n} O_p\big(tr(\mathbf{K}^{-1}_{\mathcal{W}} d\mathbf{K}_{\mathcal{W}})^2\big). \end{aligned} \tag{27}$$

  where

$$\begin{aligned} \frac{t}{\sqrt{n}} tr(\mathbf{K}^{-1}_{\mathcal{W}} d\mathbf{K}_{\mathcal{W}}) &= \frac{t}{\sqrt{n}} tr\Big(\mathbf{K}^{-1}_{\mathcal{W}}(\mathbf{K}_{\mathcal{W}}\mathbf{H}_{\mathcal{W},p} + \mathbf{H}_{\mathcal{W},p}\mathbf{K}_{\mathcal{W}} - \frac{t}{\sqrt{n}}\mathbf{H}_{\mathcal{W},p}\mathbf{K}_{\mathcal{W}}\mathbf{H}_{\mathcal{W},p})\Big) \\ &= \frac{2t}{\sqrt{n}} tr(\mathbf{H}_{\mathcal{W},p}) - \frac{t^2}{n} tr(\mathbf{K}^{-1}_{\mathcal{W}}\mathbf{H}_{\mathcal{W},p}\mathbf{K}_{\mathcal{W}}\mathbf{H}_{\mathcal{W},p}) \\ &\leq \frac{2t}{\sqrt{n}} tr(\mathbf{H}_{\mathcal{W},p}) \\ &= \frac{t}{\sqrt{n}} O_p(K). \end{aligned} \tag{28}$$

  In the above expression, the inequality follows from the fact that $\mathbf{K}^{-1}_{\mathcal{W}}\mathbf{H}_{\mathcal{W},p}\mathbf{K}_{\mathcal{W}}\mathbf{H}_{\mathcal{W},p}$ is positive semi-definite, and the last line follows from Proposition 2, i.e., $tr(\mathbf{H}_{\mathcal{W},p}) = O_p(K)$.

  By combing (27) and (28):

$$log|\mathbf{K}_{n,\mathcal{W}}| - log|\mathbf{K}_{\mathcal{W}}| = -\frac{t}{\sqrt{n}} tr(\mathbf{K}^{-1}_{\mathcal{W}} d\mathbf{K}_{\mathcal{W}}) + \frac{t^2}{n} O_p\big(tr(\mathbf{K}^{-1}_{\mathcal{W}} d\mathbf{K}_{\mathcal{W}})^2\big) = t * O_p(\frac{K}{\sqrt{n}}) = o_p(1). \tag{29}$$

  where recall $O_p(\frac{K}{\sqrt{n}}) = o_p(1)$ since $K = o_p(n^{1/2})$.

[1] For the log pseudo-determinant function $f(\mathbf{X}) = log|\mathbf{X}|$, we can compute its gradient function as $\nabla_{\mathbf{X}} f(\mathbf{X}) = \mathbf{X}^+$ Hessian $H_{\mathbf{X}} f(\mathbf{X}) = \mathbf{X}^+ \otimes \mathbf{X}^+$.

[2] The second-order term in Taylor expansion is $vec(d\mathbf{K}_{\mathcal{W}})^\top(\mathbf{K}^{-1}_{\mathcal{W}} \otimes \mathbf{K}^{-1}_{\mathcal{W}})vec(d\mathbf{K}_{\mathcal{W}})$. Using property of Kronecker product $(\mathbf{C}^\top \otimes \mathbf{A})vec(\mathbf{B}) = vec(\mathbf{ABC})$, the second-order term can also be written as $vec(d\mathbf{K}_{\mathcal{W}})^\top vec(\mathbf{K}^{-1}_{\mathcal{W}} d\mathbf{K}_{\mathcal{W}} \mathbf{K}^{-1}_{\mathcal{W}}) = tr(d\mathbf{K}_{\mathcal{W}}\mathbf{K}^{-1}_{\mathcal{W}} d\mathbf{K}_{\mathcal{W}}\mathbf{K}^{-1}_{\mathcal{W}}) = tr((\mathbf{K}^{-1}_{\mathcal{W}} d\mathbf{K}_{\mathcal{W}})^2) \leq tr(\mathbf{K}^{-1}_{\mathcal{W}} d\mathbf{K}_{\mathcal{W}})^2$, where the last inequality follows from the fact that $\mathbf{K}^{-1}_{\mathcal{W}} d\mathbf{K}_{\mathcal{W}}$ is positive semidefinite.

- Second term: $\mathbf{f}^\top\big(\mathbf{K}_{n,\mathcal{W}}^{-1} - \mathbf{K}_{\mathcal{W}}^{-1}\big)\mathbf{f}$

  Bound this term using the Cauchy-Schwarz inequality $\mathbf{f}^\top\big(\mathbf{K}_{n,\mathcal{W}}^{-1} - \mathbf{K}_{\mathcal{W}}^{-1}\big)\mathbf{f} \leq ||\mathbf{K}_{n,\mathcal{W}}^{-1} - \mathbf{K}_{\mathcal{W}}^{-1}||_\infty||\mathbf{f}||_\infty^2$, where recall $||.||_2$ denotes the matrix 2-norm, i.e., the largest singular value. Notice that by applying the inversion formula $(\mathbf{A}+\mathbf{B})^{-1} = \mathbf{A}^{-1} - \mathbf{A}^{-1}\mathbf{B}(\mathbf{A}+\mathbf{B})^{-1}$ [10], we have $\mathbf{K}_{n,\mathcal{W}}^{-1} - \mathbf{K}_{\mathcal{W}}^{-1} = \frac{t}{\sqrt{n}}(\mathbf{K}_{\mathcal{W}}^{-1}d\mathbf{K}_{\mathcal{W}})\mathbf{K}_{n,\mathcal{W}}^{-1}$, and further manipulation reveals that:

  $$\mathbf{K}_{\mathcal{W}}^{-1}d\mathbf{K}_{\mathcal{W}}\mathbf{K}_{n,\mathcal{W}}^{-1} = \mathbf{K}_{\mathcal{W}}^{-1}(\mathbf{K}_{\mathcal{W}}\mathbf{H}_{\mathcal{W},p} + \mathbf{H}_{\mathcal{W},p}\mathbf{K}_{\mathcal{W}}\mathbf{B}_{t,n})(\mathbf{B}_{t,n}^+\mathbf{K}_{\mathcal{W}}^{-1}\mathbf{B}_{t,n}^+) = \mathbf{H}_{\mathcal{W},p}\mathbf{B}_{t,n}^+\mathbf{K}_{\mathcal{W}}^{-1}\mathbf{B}_{t,n}^+ + \mathbf{K}_{\mathcal{W}}^{-1}\mathbf{H}_{\mathcal{W},p}\mathbf{B}_{t,n}^+$$

  Then, by triangular inequality, we can bound $||\mathbf{K}_{n,\mathcal{W}}^{-1}||_\infty$ as:

  $$\begin{aligned}
  ||\mathbf{K}_{n,\mathcal{W}}^{-1} - \mathbf{K}_{\mathcal{W}}^{-1}||_\infty &= \frac{t}{\sqrt{n}}||\mathbf{K}_{\mathcal{W}}^{-1}d\mathbf{K}_{\mathcal{W}}\mathbf{K}_{n,\mathcal{W}}^{-1}||_\infty \\
  &\leq \frac{t}{\sqrt{n}}\Big(||\mathbf{H}_{\mathcal{W},p}\mathbf{B}_{t,n}^+\mathbf{K}_{\mathcal{W}}^{-1}\mathbf{B}_{t,n}^+||_\infty + ||\mathbf{K}_{\mathcal{W}}^{-1}\mathbf{H}_{\mathcal{W},p}\mathbf{B}_{t,n}^+||_\infty\Big) \\
  &= \frac{t}{\sqrt{n}}\Big(||\mathbf{B}_{t,n}^+\mathbf{H}_{\mathcal{W},p}\mathbf{K}_{\mathcal{W}}^{-1}\mathbf{B}_{t,n}^+||_\infty + ||\mathbf{K}_{\mathcal{W}}^{-1}\mathbf{H}_{\mathcal{W},p}\mathbf{B}_{t,n}^+||_\infty\Big) \\
  &\leq \frac{t}{\sqrt{n}}\Big(||\mathbf{H}_{\mathcal{W},p}\mathbf{K}_{\mathcal{W}}^{-1}||_\infty||\mathbf{B}_{t,n}^+||_\infty^2 + ||\mathbf{K}_{\mathcal{W}}^{-1}\mathbf{H}_{\mathcal{W},p}||_\infty||\mathbf{B}_{t,n}^+||_\infty\Big) \\
  &= \frac{t}{\sqrt{n}}\Big(||\mathbf{H}_{\mathcal{W},p}\mathbf{K}_{\mathcal{W}}^{-1}||_\infty + ||\mathbf{K}_{\mathcal{W}}^{-1}\mathbf{H}_{\mathcal{W},p}||_\infty\Big) = \frac{2t}{\sqrt{n}}||\mathbf{K}_{\mathcal{W}}^{-1}\mathbf{H}_{\mathcal{W},p}||_\infty \\
  &\leq \frac{2t}{\sqrt{n}}||\mathbf{K}_{\mathcal{W}}^{-1}||_\infty * ||\mathbf{H}_{\mathcal{W},p}||_\infty = t * O_p(n^{-1/2}),
  \end{aligned} \tag{30}$$

  where the second equality follows since $\mathbf{H}_{\mathcal{W},p}\mathbf{B}_{t,n}^+ = \mathbf{B}_{t,n}^+\mathbf{H}_{\mathcal{W},p}$ due to the fact that $\mathbf{B}_{t,n}^+ = \mathbf{H}_{\mathcal{W},p}^+(\mathbf{H}_{\mathcal{W},p}^+ - \frac{t}{\sqrt{n}}\mathbf{I})^+ = (\mathbf{H}_{\mathcal{W},p}^+ - \frac{t}{\sqrt{n}}\mathbf{I})^+\mathbf{H}_{\mathcal{W},p}^+$. The third equality follows since $||\mathbf{B}_{t,n}^+||_\infty \leq ||\mathbf{B}_{t,n}^+||_2 = ||(\mathbf{I} - \frac{t}{\sqrt{n}}\mathbf{H}_{\mathcal{W},p})^+||_2 = 1$ due to the fact that $\mathbf{H}_{\mathcal{W},p}$ is not full-column rank, and the last line follows by the facts that $||\mathbf{K}_{\mathcal{W}}^{-1}||_\infty \leq ||\mathbf{K}_{\mathcal{W}}^{-1}||_2 = O_p(1)$ due to $\mathbf{K}_{\mathcal{W}} = \mathbf{\Phi}_{\mathcal{W}}\mathbf{\Phi}_{\mathcal{W}}^\top + \sigma_{b_0}^2\mathbf{I}$ and $||\mathbf{H}_{\mathcal{W},p}||_\infty \leq ||\mathbf{H}_{\mathcal{W},p}||_2 = o_p(1)$ due to Proposition 2.

  Finally, we know $||\mathbf{f}||_\infty^2 = C_f^2 = o_p(1)$ due to assumption that $||f_0||_\infty < C_f$ . As a result, the term $\mathbf{f}^\top\big(\mathbf{K}_{n,\mathcal{W}}^{-1} - \mathbf{K}_{\mathcal{W}}^{-1}\big)\mathbf{f}$ can be bounded as:

  $$\mathbf{f}^\top\big(\mathbf{K}_{n,\mathcal{W}}^{-1} - \mathbf{K}_{\mathcal{W}}^{-1}\big)\mathbf{f} \leq ||\mathbf{K}_{n,\mathcal{W}}^{-1} - \mathbf{K}_{\mathcal{W}}^{-1}||_\infty||\mathbf{f}||_\infty^2 = t * O_p(n^{-\frac{1}{2}}) = o_p(1). \tag{31}$$

- Third and fourth term: $\frac{t}{\sqrt{n}}\mathbf{a}_n^\top\mathbf{K}_{n,\mathcal{W}}^{-1}\mathbf{f}$ and $\frac{t^2}{2n}\mathbf{a}_n^\top\mathbf{K}_{n,\mathcal{W}}^{-1}\mathbf{a}_n^\top$.

  First notice that:

  $$||\mathbf{K}_{n,\mathcal{W}}^{-1}||_\infty = ||\mathbf{B}_{t,n}^+\mathbf{K}_{\mathcal{W}}^{-1}\mathbf{B}_{t,n}^+||_\infty \leq ||\mathbf{K}_{\mathcal{W}}^{-1}||_\infty||\mathbf{B}_{t,n}^+||_\infty^2 = ||\mathbf{K}_{\mathcal{W}}^{-1}||_\infty = O_p(1)$$

  where the second equality follows since $||\mathbf{B}_{t,n}^+||_\infty \leq ||\mathbf{B}_{t,n}^+||_2 = ||(\mathbf{I} - \frac{t}{\sqrt{n}}\mathbf{H}_{\mathcal{W},p})^+||_2 = 1$ due to the fact that $\mathbf{H}_{\mathcal{W},p}$ is not full-column rank. The final equality follows from the fact that $||\mathbf{K}_{\mathcal{W}}^{-1}||_\infty \leq |\mathbf{K}_{\mathcal{W}}^{-1}||_2 = \sigma_{b_0}^{-2} = O_p(1)$ due to $\mathbf{K}_{\mathcal{W}} = \mathbf{\Phi}_{\mathcal{W}}\mathbf{\Phi}_{\mathcal{W}}^\top + \sigma_{b_0}^2\mathbf{I}$.

  Also notice that

  $$\begin{aligned}
  ||\mathbf{a}_n||_\infty = ||\mathbf{H}_{\mathcal{W},p}(\mathbf{f}_{0,\mathcal{W}} + \omega_{\mathcal{W}})||_\infty &\leq ||\mathbf{H}_{\mathcal{W},p}||_\infty||\mathbf{f}_{0,\mathcal{W}}||_\infty + ||\omega_{\mathcal{W}}||_\infty \\
  &\leq ||\mathbf{H}_{\mathcal{W},p}||_2||\mathbf{f}_{0,\mathcal{W}}||_\infty + ||\omega_{\mathcal{W}}||_2 = O_p(1)
  \end{aligned}$$

  since $||\omega_{\mathcal{W}}||_2 = O_p(1)$, $||\mathbf{f}_{0,\mathcal{W}}||_\infty = C_f = O_p(1)$ and $||\mathbf{H}_{\mathcal{W},p}||_2 = O_p(1)$ by Proposition 2. Also

  $$||\mathbf{f}||_\infty = ||\mathbf{X}(\prod_{l=1}^{L}\mathbf{W}_l\mathbf{S}_l)\boldsymbol{\beta}||_\infty \leq ||\mathbf{X}||_\infty * \prod_{l=1}^{L}(||\mathbf{W}_l||_\infty||\mathbf{S}_l||_\infty) * ||\boldsymbol{\beta}||_\infty = O_p(1)$$

  since $||\mathbf{W}_l||_\infty \leq B \leq 1$, $||\boldsymbol{\beta}||_\infty \leq B \leq 1$, and the fact that elements in $\mathbf{X}$ and $\mathbf{S}_l$ are bounded between $(0, 1)$.

Therefore we can bound $\frac{t}{\sqrt{n}}\mathbf{a}_n^\top \mathbf{K}_{n,\mathcal{W}}^{-1}\mathbf{f}$ as:

$$\frac{t}{\sqrt{n}}\mathbf{a}_n^\top \mathbf{K}_{n,\mathcal{W}}^{-1}\mathbf{f} \leq \frac{t}{\sqrt{n}}||\mathbf{a}_n||_\infty||\mathbf{K}_{n,\mathcal{W}}^{-1}||_\infty||\mathbf{f}||_\infty \leq t * O_p(n^{-\frac{1}{2}}) = o_p(1). \tag{32}$$

Similarly, we can bound the fourth term $\frac{t^2}{2n}\mathbf{a}_n^\top \mathbf{K}_{n,\mathcal{W}}^{-1}\mathbf{a}_n^\top$ as:

$$\frac{t^2}{2n}\mathbf{a}_n^\top \mathbf{K}_{n,\mathcal{W}}^{-1}\mathbf{a}_n^\top \leq \frac{t^2}{2n}||\mathbf{a}_n||_\infty^2||\mathbf{K}_{n,\mathcal{W}}^{-1}||_\infty \leq t^2 * O_p(n^{-1}) = o_p(1). \tag{33}$$

Consequently, by combining the asymptotic bounds for the four terms (29), (31), (32) and (33), we have that

$$\mathcal{J}_n = \frac{\int e^{l_n(f_t)-l_n(f_{0,\mathcal{W}})} * e^{-\mathcal{L}_{t,n}}\, d\Pi(f_t|\mathcal{W})}{\int e^{l_n(f)-l_n(f_{0,\mathcal{W}})} d\Pi(f|\mathcal{W})} = e^{-\frac{t}{\sqrt{n}}o_p(K)} \to 1,$$

where the last equality follows since $K/\sqrt{n} = o_p(1)$ due to Assumption (1).

□

### D.2 Proof for Theorem C.3

*Proof.* Our goal is to show the asymptotic normality

$$\Pi_n\big(\sqrt{n}(\psi_{\mathcal{W}}^c(f) - \hat{\psi}_{\mathcal{W}}^c)\big|\mathcal{W}\big) \rightsquigarrow MVN(0, V_{0,\mathcal{W}}).$$

First derive the expressions for $f_t, \hat{\psi}_{\mathcal{W}}, V_{0,n}$ and $\mathcal{I}_n$. For $t = [t_1, \ldots, t_P] \in \mathbb{R}^P$, the expression for $f_t$ is:

$$\begin{aligned} f_t &= f - \frac{t^\top}{\sqrt{n}}\Big(\psi_1 + \frac{1}{2}\psi_2(f - f_{0,\mathcal{W}})\Big) - \frac{t^\top}{2n}\psi_2(\omega_{\mathcal{W}}) \\ &= \Big(I - \frac{t^\top}{\sqrt{n}} * H_{\mathcal{W}}\Big)(f) - \frac{t^\top}{\sqrt{n}} * H_{\mathcal{W}}\big(f_{0,\mathcal{W}} + \omega_{\mathcal{W}}\big). \end{aligned} \tag{34}$$

The expressions for $\hat{\psi}_{\mathcal{W}}$ and $t^\top V_{0,n}t$ are:

$$\begin{aligned} \hat{\psi}_{\mathcal{W}} &= \hat{\psi}(f_{0,\mathcal{W}}) + \frac{W_n(\psi_1)}{\sqrt{n}} + \frac{1}{2}\frac{\langle \omega_{\mathcal{W}}, \psi_2(\omega_{\mathcal{W}})\rangle_n}{n} \\ &= \hat{\psi}(f_{0,\mathcal{W}}) + 2\langle H_{\mathcal{W}}f_{0,\mathcal{W}}, \omega_{\mathcal{W}}\rangle_n + \langle H_{\mathcal{W}}\omega_{\mathcal{W}}, \omega_{\mathcal{W}}\rangle_n, \\ t^\top V_{0,n}t &= \Big|\Big|t^\top(\psi_1 - \frac{1}{2}\frac{\psi_2(\omega_{\mathcal{W}})}{\sqrt{n}})\Big|\Big|_n^2 = 4 * \Big|\Big|t^\top H_{\mathcal{W}}f_{0,\mathcal{W}} + o_p(1)\Big|\Big|_n^2, \end{aligned}$$

and the expression for $\mathcal{I}_n$ is:

$$\mathcal{I}_n = \frac{\int_{A_n} e^{l_n(f_t)-l_n(f_{0,\mathcal{W}})} d\Pi(f|\mathcal{W})}{\int_{A_n} e^{l_n(f)-l_n(f_{0,\mathcal{W}})} d\Pi(f|\mathcal{W})}.$$

It then follows from the Theorem C.1 that

$$E_n(e^{t^\top\sqrt{n}(\psi_{\mathcal{W}}^c(f)-\hat{\psi}_{\mathcal{W}}^c)}|A_n, \mathcal{W}) = e^{o_p(1)+t^\top V_{0,n}t/2} * \mathcal{I}_n.$$

Therefore to show asymptotic normality, we only need to show $\mathcal{I}_n \to 1$ for some suitable choice of $A_n$ so that $E_n(e^{t^\top\sqrt{n}(\hat{\psi}_p^c(f)-\hat{\psi}^c)}|A_n, \mathcal{W}) \to e^{t^\top V_{0,\mathcal{W}}t/2}$.

To this end, we consider the standard choice $A_n = \Big\{f\Big|||f - f_{0,\mathcal{W}}||_n \leq M_n\epsilon_n\Big\}$ for some sufficiently large $M_n \to \infty$ and $\epsilon_n$ the given rate of posterior convergence. Similar to the proof for Theorem C.1, it is sufficient to show the terms $\mathcal{J}_n \to 1$ and $\mathcal{K}_n \to 1$, where

$$\mathcal{J}_n = \frac{\int e^{l_n(f_t)-l_n(f_{0,\mathcal{W}})} d\Pi(f|\mathcal{W})}{\int e^{l_n(f)-l_n(f_{0,\mathcal{W}})} d\Pi(f|\mathcal{W})}, \quad \mathcal{K}_n = \frac{\int_{f\in A_n} e^{l_n(f_t)-l_n(f_{0,\mathcal{W}})} d\Pi(f|\mathcal{W})}{\int e^{l_n(f_t)-l_n(f_{0,\mathcal{W}})} d\Pi(f|\mathcal{W})}.$$

The argument for $\mathcal{K}_n \to 1$ is essentially the same as those in the proof for Theorem C.2 (i.e., (25)). We show $\mathcal{J}_n \to 1$ by performing change of variables $f \to f_t$ on the numerator, and then analyze the asymptotic behavior of the resulting expression. Similar to the proof for Theorem C.1, by noticing the conditional prior $\Pi(f|\mathcal{W})$ is a Gaussian process prior with kernel matrix $\mathbf{K}_{\mathcal{W}} = \mathbf{\Phi}_{\mathcal{W}}\mathbf{\Phi}_{\mathcal{W}}^\top + \sigma_{b_0}^2\mathbf{I}$ for $\mathbf{\Phi}_{n\times K} = \mathbf{X}(\prod_{l=1}^L \mathbf{W}_l\mathbf{S}_l)$, we see that given observations $\{y_i, \mathbf{x}_i\}_{i=1}^n$, the conditional prior distribution for $\mathbf{f} = [f(\mathbf{x}_1), \dots, f(\mathbf{x}_n)]^\top \in \mathbb{R}^n$ is a multivariate Gaussian with covariance matrix $\mathbf{K}_{\mathcal{W}}$:

$$d\Pi(\mathbf{f}|\mathcal{W}) \propto |\mathbf{K}_{\mathcal{W}}|^{-\frac{1}{2}} e^{-\frac{1}{2}\mathbf{f}^\top\mathbf{K}_{\mathcal{W}}^{-1}\mathbf{f}}.$$

To perform change of variable, we denote $\mathbf{f}_t \in \mathbb{R}^n$ as $f_t$ in (34) evaluated at $\{y_i, \mathbf{x}_i\}_{i=1}^n$, we can write $\mathbf{f}_t = \mathbf{B}_{t,n}\mathbf{f} - \frac{1}{\sqrt{n}}\mathbf{a}_n$ such that

$$\begin{aligned} d\Pi(\mathbf{f}_t|\mathcal{W}) &\propto |\mathbf{K}_{n,\mathcal{W}}|^{-\frac{1}{2}} e^{-\frac{1}{2}(\mathbf{f}+\frac{1}{\sqrt{n}}\mathbf{a}_n)^\top\mathbf{K}_{n,\mathcal{W}}^{-1}(\mathbf{f}+\frac{1}{\sqrt{n}}\mathbf{a}_n)} \\ &= d\Pi(\mathbf{f}|\mathcal{W}) * exp\Big[-\frac{1}{2}log\Big(\frac{|\mathbf{K}_{n,\mathcal{W}}|}{|\mathbf{K}_{\mathcal{W}}|}\Big) - \frac{1}{2}\mathbf{f}^\top\big(\mathbf{K}_{n,\mathcal{W}}^{-1} - \mathbf{K}_{\mathcal{W}}^{-1}\big)\mathbf{f} + \frac{1}{\sqrt{n}}\mathbf{a}_n^\top\mathbf{K}_{n,\mathcal{W}}^{-1}\mathbf{f} - \frac{1}{2n}\mathbf{a}_n^\top\mathbf{K}_{n,\mathcal{W}}^{-1}\mathbf{a}_n^\top\Big] \end{aligned}$$

where $\mathbf{B}_{t,n} = \mathbf{I} - \frac{1}{\sqrt{n}}\mathbf{H}_t$, $\mathbf{a}_n = \mathbf{H}_t\big(\mathbf{f}_{0,\mathcal{W}} + \omega_{\mathcal{W}}\big)$ for $\mathbf{H}_t = \sum_{p=1}^P t_p\mathbf{H}_p$, and

$$\mathbf{K}_{n,\mathcal{W}} = \mathbf{B}_{t,n}\mathbf{K}_{\mathcal{W}}\mathbf{B}_{t,n} = \mathbf{K}_{\mathcal{W}} - \frac{1}{\sqrt{n}}\Big[\mathbf{K}_{\mathcal{W}}\mathbf{H}_t + \mathbf{H}_t\mathbf{K}_{\mathcal{W}}\mathbf{B}_{t,n}\Big] = \mathbf{K}_{\mathcal{W}} - \frac{1}{\sqrt{n}}d\mathbf{K}_{\mathcal{W}},$$

where we have denoted $d\mathbf{K}_{\mathcal{W}} = \mathbf{K}_{\mathcal{W}}\mathbf{H}_t + \mathbf{H}_t\mathbf{K}_{\mathcal{W}}\mathbf{B}_{t,n}$.

Consequently, the expression of $\mathcal{J}_n$ after the change of variable becomes:

$$\mathcal{J}_n = \frac{\int e^{l_n(f_t) - l_n(f_{0,\mathcal{W}})} * e^{-\mathcal{L}_{t,n}}\, d\Pi(f_t|\mathcal{W})}{\int e^{l_n(f) - l_n(f_{0,\mathcal{W}})} d\Pi(f|\mathcal{W})},$$

where

$$\mathcal{L}_{t,n} = \frac{1}{2}log\Big(\frac{|\mathbf{K}_{n,\mathcal{W}}|}{|\mathbf{K}_{\mathcal{W}}|}\Big) + \frac{1}{2}\mathbf{f}^\top\big(\mathbf{K}_{n,\mathcal{W}}^{-1} - \mathbf{K}_{\mathcal{W}}^{-1}\big)\mathbf{f} - \frac{1}{\sqrt{n}}\mathbf{a}_n^\top\mathbf{K}_{n,\mathcal{W}}^{-1}\mathbf{f} + \frac{t^2}{2n}\mathbf{a}_n^\top\mathbf{K}_{n,\mathcal{W}}^{-1}\mathbf{a}_n^\top. \quad (35)$$

Therefore in order to show $\mathcal{J}_n \to 1$, it is sufficient to show that all terms in $\mathcal{L}_{t,n}$ are asymptotically vanishing toward zero as $n \to \infty$. Now only left to show that all the four terms in (35) are asymptotically vanishing toward zero. However, notice that the only difference between (35) and its counterpart (23) in the proof of Theorem C.2 is that $\mathbf{H}_p$ is replaced by $\mathbf{H}_t = \sum_{p=1}^P t_p\mathbf{H}_p$. Furthermore, for fixed $t$, the asymptotic behavior of $\mathbf{H}_p$ and $\mathbf{H}_t$ are similar in the sense that $tr(\mathbf{H}_t) = O_p(K)$ and $||\mathbf{H}_t||_2 = O_p(1)$ since $P = O(1)$. Therefore we can follow exactly the same arguments as those in the proof for Theorem C.2 to show all the four terms asymptotically vanishing towards zero. Consequently, we have that $\mathcal{J}_n = \frac{\int e^{l_n(f_t) - l_n(f_{0,\mathcal{W}}) + o_p(1)}\, d\Pi(f_t|\mathcal{W})}{\int e^{l_n(f) - l_n(f_{0,\mathcal{W}})} d\Pi(f|\mathcal{W})} \to 1.$.

It then follows by the semi-parametric BvM theorem (Theorem C.1) that the posterior distribution of $\sqrt{n}(\psi_{\mathcal{W}}^c(f) - \hat{\psi}_{\mathcal{W}}^c)$ converge toward a normal law with mean zero and variance $V_0$, i.e.

$$\Pi\Big(\sqrt{n}(\psi_{\mathcal{W}}^c(f) - \hat{\psi}_{\mathcal{W}}^c)\Big|\{\mathbf{x}_i, y_i\}_{i=1}^n\Big) \rightsquigarrow N(0, V_0), \quad (36)$$

where $V_0$ is the $P \times P$ matrix that takes value $t^\top V_{0,n} t = 4 * ||t^\top H_{\mathcal{W}} f_{0,\mathcal{W}}||_n^2$ for any $t \in \mathbb{R}^P$. Specifically, the matrix $V_0$ whose $(p_1, p_2)^{th}$ entry defined as $4\langle H_{p_1} f_{0,\mathcal{W}}, H_{p_2} f_{0,\mathcal{W}}\rangle_n$ will satisfy this choice. □

## E Lemmas and Propositions

**Proposition 1** (Posterior Concentration for $f_0 \in \mathcal{F}$)**.** *For the space of ReLU network $\mathcal{F} = \mathcal{F}(L, K, S, B)$ . Assuming*

- *The model architecture satisfies:*
$$L = O\big(log(N)\big), \quad K = O\big(N\big), \quad S = O\big(N\, log(N)\big).$$
*where $N \in \mathbb{N}$ is a function of sample size $n$ such that $log(N) \geq \sqrt{log(n)}$.*

- *The prior distribution $\Pi(\mathcal{W})$ is an i.i.d. product of Gaussian distributions.*

*Then, for $f_0 \in \mathcal{F}$, the posterior distribution $\Pi_n(f) = \Pi(f|\{\mathbf{x}_i, y_i\}_{i=1}^n)$ contracts toward $f_0$ in a rate of at least $\epsilon_n = O\big((N/n) * log(N)^3\big)$, i.e., for any $M_n \to \infty$*
$$E_0\Pi_n(||f - f_0||_n^2 \geq M_n\epsilon_n) \to 0$$
*In particular, if $N = o_p(n^{1/2})$ (i.e. Assumption 1), we then have $\epsilon_n = O\big(n^{-1/2} * log(n)^3\big)$.*

*Proof.* We show posterior consistency by invoking Theorem 1 of [9]. As argued in [17] (Proof for Theorem 6.1), it is sufficient to show below two conditions about the prior distribution:
$$logN(\epsilon_n, \mathcal{F}, ||.||_\infty) \leq Cn\epsilon_n \tag{37}$$
$$\Pi\Big(||f - f_0||_\infty^2 \leq \epsilon_n\Big) \geq e^{-Cn\epsilon_n} \tag{38}$$
where $C > 1$ is an universal constant. The first condition (37) ensures the model size, which is measured by the covering number of $\mathcal{F}$ (i.e., the minimal number of $||.||_\infty$-balls with radius $\delta$ that covers $\mathcal{F}$) is not too large. The second condition (38) ensures the model 's prior distribution places sufficient prior mass around the target function $f_0$. For the rest of this proof, we show the statement of interest by showing these two conditions.

- **Entropy Condition**: $logN(\epsilon_n, \mathcal{F}, ||.||_n) \leq n\epsilon_n$

  We show this condition by invoking the classic result on the covering number of neural network approximation spaces (Lemma 2) [1] . Specifically, by setting $\delta = \epsilon_n$ in Lemma 3, we have
$$\begin{aligned} logN(\epsilon_n, \mathcal{F}, ||.||_\infty) &\leq S\, log(\epsilon_n^{-1} L(K+1)^{2L}) \\ &\lesssim S\, log(\epsilon_n^{-1}) + S\, L\, log(K) \\ &\lesssim N\, log(N)\, log(\frac{n}{Nlog(N)^3}) + Nlog(N)^3 \\ &\lesssim N\, log(N)\, (log(n) + log(N)^2) \\ &\lesssim N\, log(N)^3 = n\epsilon_n \end{aligned}$$
  where the last line follows from the assumption that $log(N) \geq \sqrt{log(n)}$ and the definition of $\epsilon_n$.

- **Prior Mass Condition**: $\Pi\Big(||f - f_0||_n \leq \epsilon_n\Big) \geq e^{-Cn\epsilon_n}$.

  We show this using the classic concentration inequality for the centered Gaussian measure $\Pi$ (Lemma 1). First notice that as argued in the proof of Theorem 6.1 of [17], by the proof of Lemma 5 of [20]:
$$\Big\{f\Big|||f - f_0||_\infty^2 \leq \epsilon_n\Big\} \subset \Big\{\mathcal{W}\Big|||\mathcal{W} - \mathcal{W}_0||_\infty^2 \leq \frac{\epsilon_n}{(V(L+1))^2}\Big\}$$
  where $V = O\big(P * K^L\big)$. Therefore
$$\begin{aligned} \Pi\Big(||f - f_0||_\infty^2 \leq \epsilon_n\Big) &\geq \Pi\Big(||\mathcal{W} - \mathcal{W}_0||_\infty^2 \leq \frac{\epsilon_n}{(V(L+1))^2}\Big) \\ &\geq exp\Big(-\frac{||\mathcal{W}_0||_\Pi^2}{2}\Big)\Pi\Big(||\mathcal{W}||_\infty^2 < \frac{\epsilon_n}{(V(L+1))^2}\Big) \\ &\geq exp\Big(-\frac{||\mathcal{W}_0||_\Pi^2}{2}\Big)exp\Big(-\frac{\epsilon_n}{(V(L+1))^2}\Big) \\ &\geq exp(-Cn\epsilon_n) \end{aligned}$$

for some $C > 1$. In the above expression, the second inequality follows from Lemma 1, and the third inequality follows from the Borell's inequality [23].

**Proposition 2.** *Recall that a ReLU network $f \in \mathcal{F}(L, K, S, B)$ adopts basis function representation $f(\mathbf{x}) = \sum_{k=1}^{K} \beta_k \phi_k(\mathbf{x}) = \boldsymbol{\phi}(\mathbf{x})^\top \boldsymbol{\beta}$ at the output layer. Denote $\boldsymbol{\Phi}$ and $\partial_p \boldsymbol{\Phi}$ the $n \times K$ matrices of $\boldsymbol{\phi}$ and $\frac{\partial}{\partial x_p} \boldsymbol{\phi}$ evaluated at observations $\{\mathbf{x}_i, y_i\}_{i=1}^n$, such that $\boldsymbol{\Phi}_{n\times K} = \mathbf{X}\mathbf{W}_1\mathbf{S}_1(\prod_{l=2}^{L}\mathbf{W}_l\mathbf{S}_l)$ and $\partial_p\boldsymbol{\Phi}_{n\times K} = \mathbf{W}_{1,p}\mathbf{S}_1(\prod_{l=1}^{L}\mathbf{W}_l\mathbf{S}_l)$. Denote*

$$\mathbf{H}_p = (\boldsymbol{\Phi}^+)^\top \partial_p \boldsymbol{\Phi}^\top \partial_p \boldsymbol{\Phi} \boldsymbol{\Phi}^+$$

*where $\boldsymbol{\Phi}^+_{K\times n}$ is the generalized inverse of $\boldsymbol{\Phi}_{n\times K}$. Then:*

$$||\mathbf{H}_p||_2 = O_p(1), \quad tr(\mathbf{H}_p) = O_p(K),$$

*Proof.* Notice that $||\mathbf{H}_p||_2 = O_p(1)$ implies $tr(\mathbf{H}_p) = O_P(K)$ since

$$tr(\mathbf{H}_p) \leq rank(\mathbf{H}_p) * ||\mathbf{H}||_2 = O_p(rank(\mathbf{H}_p)) = O_p(K).$$

Therefore we only need to show $||\mathbf{H}||_2 = O_p(1)$.

Show $||\mathbf{H}_p||_2 = O_p(1)$ by showing that it is upper bounded by certain constant that does not depend on $n$. Recall that $\mathbf{H}_p = (\boldsymbol{\Phi}^+)^\top(\partial_p\boldsymbol{\Phi}^\top\partial_p\boldsymbol{\Phi})\boldsymbol{\Phi}^+$, by the fact that 2-norm is invariant under cyclic permutations, we then have

$$\begin{aligned}||\mathbf{H}_p||_2 &= ||(\partial_p\boldsymbol{\Phi}\boldsymbol{\Phi}^+)^\top(\partial_p\boldsymbol{\Phi}\boldsymbol{\Phi}^+)||_2 = ||\partial_p\boldsymbol{\Phi}(\boldsymbol{\Phi}^+\boldsymbol{\Phi}^{+\top})\partial_p\boldsymbol{\Phi}^\top||_2 = ||\partial_p\boldsymbol{\Phi}(\boldsymbol{\Phi}^\top\boldsymbol{\Phi})^{-1}\partial_p\boldsymbol{\Phi}^\top||_2\\ &= ||(\boldsymbol{\Phi}^\top\boldsymbol{\Phi})^{-1}(\partial_p\boldsymbol{\Phi}^\top\partial_p\boldsymbol{\Phi})||_2\end{aligned}$$

Denote $\mathbf{M} = \mathbf{S}_1(\prod_{l=2}^{L}\mathbf{W}_l\mathbf{S}_l)$, then we have $\boldsymbol{\Phi} = \mathbf{X}\mathbf{W}_1\mathbf{M}$ and $\partial_p\boldsymbol{\Phi} = \mathbf{W}_{1,p}\mathbf{M}$. Denote $\mathbf{X}_p = diag(x_{1,p}, x_{2,p}, \dots, x_{n,p})$ and notice that $\mathbf{X}\mathbf{W}_1 = \sum_p \mathbf{X}_p\mathbf{W}_{1,p}$, so we see that $\boldsymbol{\Phi}$ is related to $\partial_p\boldsymbol{\Phi}$ through the expression $\boldsymbol{\Phi} = \sum_p \mathbf{X}_p\partial_p\boldsymbol{\Phi}$, and

$$\boldsymbol{\Phi}^\top\boldsymbol{\Phi} = (\sum_p \mathbf{X}_p\partial_p\boldsymbol{\Phi})^\top(\sum_p \mathbf{X}_p\partial_p\boldsymbol{\Phi}) = \sum_{p_1,p_2}\partial_{p_1}\boldsymbol{\Phi}^\top\mathbf{X}_{p_1}\mathbf{X}_{p_2}\partial_{p_2}\boldsymbol{\Phi}.$$

Using the inversion formula $(\mathbf{A}+\mathbf{B})^{-1} = (\mathbf{I}+\mathbf{A}^{-1}\mathbf{B})^{-1}\mathbf{A}^{-1}$ [10], we can write $(\boldsymbol{\Phi}^\top\boldsymbol{\Phi})^{-1}$ as:

$$\begin{aligned}(\boldsymbol{\Phi}^\top\boldsymbol{\Phi})^{-1} &= \Big(\partial_p\boldsymbol{\Phi}^\top\mathbf{X}_p^2\partial_p\boldsymbol{\Phi} + \sum_{p_1,p_2\neq p}\partial_{p_1}\boldsymbol{\Phi}^\top\mathbf{X}_{p_1}\mathbf{X}_{p_2}\partial_{p_2}\boldsymbol{\Phi}\Big)^{-1}\\ &= \Big(\mathbf{I} + (\partial_p\boldsymbol{\Phi}^\top\mathbf{X}_p^2\partial_p\boldsymbol{\Phi})^{-1}\sum_{p_1,p_2\neq p}\partial_{p_1}\boldsymbol{\Phi}^\top\mathbf{X}_{p_1}\mathbf{X}_{p_2}\partial_{p_2}\boldsymbol{\Phi}\Big)^{-1}(\partial_p\boldsymbol{\Phi}^\top\mathbf{X}_p^2\partial_p\boldsymbol{\Phi})^{-1}.\end{aligned}$$

Consequently, we can bound $||\mathbf{H}_p||_2$ as:

$$\begin{aligned}||\mathbf{H}_p||_2 &= ||(\boldsymbol{\Phi}^\top\boldsymbol{\Phi})^{-1}(\partial_p\boldsymbol{\Phi}^\top\partial_p\boldsymbol{\Phi})||_2\\ &= \Big|\Big|\Big(\mathbf{I} + (\partial_p\boldsymbol{\Phi}^\top\mathbf{X}_p^2\partial_p\boldsymbol{\Phi})^{-1}\sum_{p_1,p_2\neq p}\partial_{p_1}\boldsymbol{\Phi}^\top\mathbf{X}_{p_1}\mathbf{X}_{p_2}\partial_{p_2}\boldsymbol{\Phi}\Big)^{-1}(\partial_p\boldsymbol{\Phi}^\top\mathbf{X}_p^2\partial_p\boldsymbol{\Phi})^{-1}(\partial_p\boldsymbol{\Phi}^\top\partial_p\boldsymbol{\Phi})\Big|\Big|_2\\ &\leq \Big|\Big|\Big(\mathbf{I} + (\partial_p\boldsymbol{\Phi}^\top\mathbf{X}_p^2\partial_p\boldsymbol{\Phi})^{-1}\sum_{p_1,p_2\neq p}\partial_{p_1}\boldsymbol{\Phi}^\top\mathbf{X}_{p_1}\mathbf{X}_{p_2}\partial_{p_2}\boldsymbol{\Phi}\Big)^{-1}\Big|\Big|_2 * \Big|\Big|(\partial_p\boldsymbol{\Phi}^\top\mathbf{X}_p^2\partial_p\boldsymbol{\Phi})^{-1}(\partial_p\boldsymbol{\Phi}^\top\partial_p\boldsymbol{\Phi})\Big|\Big|_2\end{aligned}$$

Notice in the last line of the above expression, the first term can be bounded as:

$$\Big|\Big|\Big(\mathbf{I} + (\partial_p\boldsymbol{\Phi}^\top\mathbf{X}_p^2\partial_p\boldsymbol{\Phi})^{-1}\sum_{p_1,p_2\neq p}\partial_{p_1}\boldsymbol{\Phi}^\top\mathbf{X}_{p_1}\mathbf{X}_{p_2}\partial_{p_2}\boldsymbol{\Phi}\Big)^{-1}\Big|\Big|_2 \leq 1 \qquad (39)$$

This is because $\lambda_{\min}\Big(\mathbf{I} + (\partial_p \boldsymbol{\Phi}^\top \mathbf{X}_p^2 \partial_p \boldsymbol{\Phi})^{-1} \sum_{p_1, p_2 \neq p} \partial_{p_1} \boldsymbol{\Phi}^\top \mathbf{X}_{p_1} \mathbf{X}_{p_2} \partial_{p_2} \boldsymbol{\Phi}\Big) \geq 1$ due to the fact that $\partial_{p_1} \boldsymbol{\Phi}^\top \mathbf{X}_{p_1} \mathbf{X}_{p_2} \partial_{p_2} \boldsymbol{\Phi}$ is full column rank for all $p_1, p_2$, which implies that $\lambda_{\max}$ of (39) is no larger than 1.

The second term can be bounded as:

$$\begin{aligned}
||(\partial_p \boldsymbol{\Phi}^\top \mathbf{X}_p^2 \partial_p \boldsymbol{\Phi})^{-1} (\partial_p \boldsymbol{\Phi}^\top \partial_p \boldsymbol{\Phi})||_2 &= ||(\partial_p \boldsymbol{\Phi}^+ \mathbf{X}_p^{-2} \partial_p \boldsymbol{\Phi}^{+\top})(\partial_p \boldsymbol{\Phi}^\top \partial_p \boldsymbol{\Phi})||_2 \\
&= ||\partial_p \boldsymbol{\Phi}^+ \mathbf{X}_p^{-2} \partial_p \boldsymbol{\Phi}||_2 \\
&= ||\mathbf{X}_p^{-2} \partial_p \boldsymbol{\Phi} \partial_p \boldsymbol{\Phi}^+||_2 \\
&\leq ||\mathbf{X}_p^{-2}||_2 ||\partial_p \boldsymbol{\Phi} \partial_p \boldsymbol{\Phi}^+||_2 \\
&= ||\mathbf{X}_p^{-1}||_2^2, \qquad (40)
\end{aligned}$$

where we have denoted $\boldsymbol{\Phi}^+ = \mathbf{V}\mathbf{D}^{-1}\mathbf{U}^\top$ for $\boldsymbol{\Phi} = \mathbf{U}\mathbf{D}\mathbf{V}^\top$. In above expression, the third equality follows from the fact that the eigenvalue of the product of square matrices is invariant under cyclic permutation of the product order [13].

Combining (39) and (40), we have:

$$\begin{aligned}
||\mathbf{H}_p||_2 &= ||(\boldsymbol{\Phi}^\top \boldsymbol{\Phi})^{-1} (\partial_p \boldsymbol{\Phi}^\top \partial_p \boldsymbol{\Phi})||_2 \\
&\leq \Big|\Big|\Big(\mathbf{I} + (\partial_p \boldsymbol{\Phi}^\top \mathbf{X}_p^2 \partial_p \boldsymbol{\Phi})^{-1} \sum_{p_1, p_2 \neq p} \partial_{p_1} \boldsymbol{\Phi}^\top \mathbf{X}_{p_1} \mathbf{X}_{p_2} \partial_{p_2} \boldsymbol{\Phi}\Big)^{-1}\Big|\Big|_2 * \Big|\Big|(\partial_p \boldsymbol{\Phi}^\top \mathbf{X}_p^2 \partial_p \boldsymbol{\Phi})^{-1} (\partial_p \boldsymbol{\Phi}^\top \partial_p \boldsymbol{\Phi})\Big|\Big|_2 \\
&\leq ||\mathbf{X}_p^{-1}||_2^2
\end{aligned}$$

Recall that since $\mathbf{X}_p = diag(\mathbf{x}_{1,p}, x_{2,p}, \ldots, x_{n,p})$ is a diagonal matrix, we have $||\mathbf{X}_p^{-1}||_2 = max(1/x_{i,p}) = 1/min(x_{i,p}) \leq 1/c_x$, i.e. bounded by a constant that does not depend on $n$. Therefore $||\mathbf{H}_p||_2 = O_p(1)$. □

**Lemma 1** (Gaussian Shift-ball Inequality). *Let $\Pi(f)$ be a centered Gaussian measure and $H_\Pi$ the Hilbert space induced by $\Pi$ with norm $||.||_\Pi$. For $f_0 \in H_\Pi$, it holds that*

$$\Pi(||f - f_0||_\infty \leq \delta) \geq exp(-\frac{||f_0||_\Pi^2}{2})\Pi(||f||_\infty < \delta)$$

*Proof.* [12], Theorem 2

**Lemma 2** (Covering Number for $\mathcal{F}(L, K, S, B)$). *For the space of ReLU network $\mathcal{F} = \mathcal{F}(L, K, S, B)$ as defined in (2), denote the covering number of $\mathcal{F}$ as $N(\delta, \mathcal{F}, ||.||_\infty)$, i.e., the minimal number of $||.||_\infty$-balls with radius $\delta$ that covers $\mathcal{F}$, can be bounded as:*

$$logN(\delta, \mathcal{F}, ||.||_\infty) \leq S\, log(\delta^{-1} L (K+1)^{2L})$$

*Proof.* Lemma 3 of [21], where we take $B \leq 1$ due to assumption in (2).

## References


[1] M. Anthony. *Neural Network Learning: Theoretical Foundations*. Cambridge University Press, Cambridge, 1 edition edition, Aug. 2009.

[2] F. Bach. Breaking the Curse of Dimensionality with Convex Neural Networks. *arXiv:1412.8690 [cs, math, stat]*, Dec. 2014. arXiv: 1412.8690.

[3] A. Berlinet and C. Thomas-Agnan. *Reproducing Kernel Hilbert Spaces in Probability and Statistics*. Springer, Boston, 2004 edition edition, Dec. 2003.

[4] P. J. Bickel and B. J. K. Kleijn. The semiparametric Bernstein–von Mises theorem. *The Annals of Statistics*, 40(1):206–237, Feb. 2012.

[5] I. Castillo. A semiparametric Bernstein–von Mises theorem for Gaussian process priors. *Probability Theory and Related Fields*, 152(1):53–99, Feb. 2012.

[6] I. Castillo and R. Nickl. Nonparametric Bernstein–von Mises theorems in Gaussian white noise. *The Annals of Statistics*, 41(4):1999–2028, Aug. 2013.

[7] I. Castillo and J. Rousseau. A Bernstein–von Mises theorem for smooth functionals in semiparametric models. *The Annals of Statistics*, 43(6):2353–2383, Dec. 2015.

[8] D. Freedman. Wald Lecture: On the Bernstein-von Mises theorem with infinite-dimensional parameters. *The Annals of Statistics*, 27(4):1119–1141, Aug. 1999.

[9] S. Ghosal, J. K. Ghosh, and A. W. v. d. Vaart. Convergence rates of posterior distributions. *The Annals of Statistics*, 28(2):500–531, Apr. 2000.

[10] H. V. Henderson and S. R. Searle. On Deriving the Inverse of a Sum of Matrices. *SIAM Review*, 23(1):53–60, 1981.

[11] A. Holbrook. Differentiating the pseudo determinant. *arXiv:1802.04878 [stat]*, Feb. 2018. arXiv: 1802.04878.

[12] J. Kuelbs, W. V. Li, and W. Linde. The Gaussian measure of shifted balls. *Probability Theory and Related Fields*, 98(2):143–162, June 1994.

[13] J. K. Merikoski and R. Kumar. Inequalities for spreads of matrix sums and products. In *Applied Mathematics E-Notes, 4:150 – 159*, 2004.

[14] R. M. Neal. *Bayesian Learning for Neural Networks*. Lecture Notes in Statistics. Springer-Verlag, New York, 1996.

[15] A. Rahimi and B. Recht. Weighted Sums of Random Kitchen Sinks: Replacing minimization with randomization in learning. In D. Koller, D. Schuurmans, Y. Bengio, and L. Bottou, editors, *Advances in Neural Information Processing Systems 21*, pages 1313–1320. Curran Associates, Inc., 2009.

[16] V. Rivoirard and J. Rousseau. Bernstein–von Mises theorem for linear functionals of the density. *The Annals of Statistics*, 40(3):1489–1523, June 2012.

[17] V. Rockova and N. Polson. Posterior Concentration for Sparse Deep Learning. In S. Bengio, H. Wallach, H. Larochelle, K. Grauman, N. Cesa-Bianchi, and R. Garnett, editors, *Advances in Neural Information Processing Systems 31*, pages 930–941. Curran Associates, Inc., 2018.

[18] L. Rosasco, S. Villa, S. Mosci, M. Santoro, and A. Verri. Nonparametric Sparsity and Regularization. *Journal of Machine Learning Research*, 14:1665–1714, 2013.

[19] J. Rousseau. On the Frequentist Properties of Bayesian Nonparametric Methods. *Annual Review of Statistics and Its Application*, 3(1):211–231, June 2016.

[20] J. Schmidt-Hieber. Nonparametric regression using deep neural networks with ReLU activation function. *arXiv:1708.06633 [cs, math, stat]*, Aug. 2017. arXiv: 1708.06633.

[21] T. Suzuki. Adaptivity of deep ReLU network for learning in Besov and mixed smooth Besov spaces: optimal rate and curse of dimensionality. Sept. 2018.

[22] A. van der Vaart and H. van Zanten. Rates of contraction of posterior distributions based on Gaussian process priors. *The Annals of Statistics*, 36(3):1435–1463, June 2008.

[23] A. W. van der Vaart and J. H. van Zanten. Reproducing kernel Hilbert spaces of Gaussian priors. *arXiv:0805.3252 [math, stat]*, pages 200–222, 2008. arXiv: 0805.3252.
